# Supplementary material for: A tutorial on individualized treatment effect prediction from randomized trials with a binary endpoint
Source: arXiv:2106.05588 ancillary file (2021-06-10)

$\beta_t < 0$ , HOM, N=400

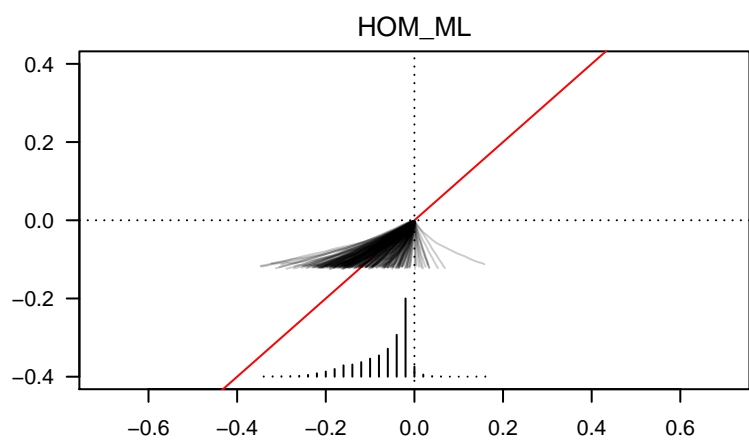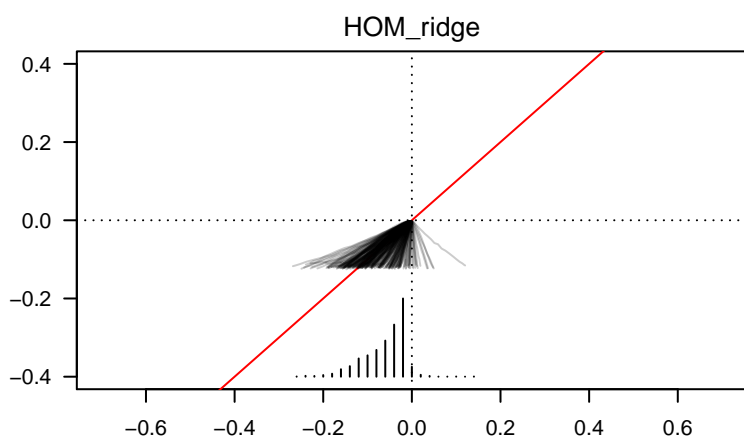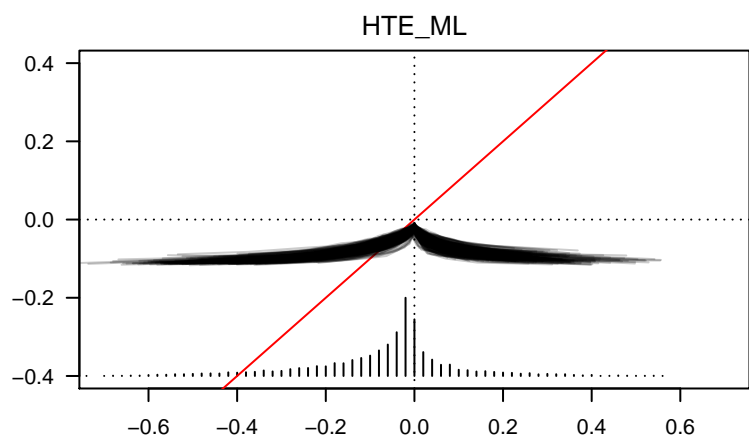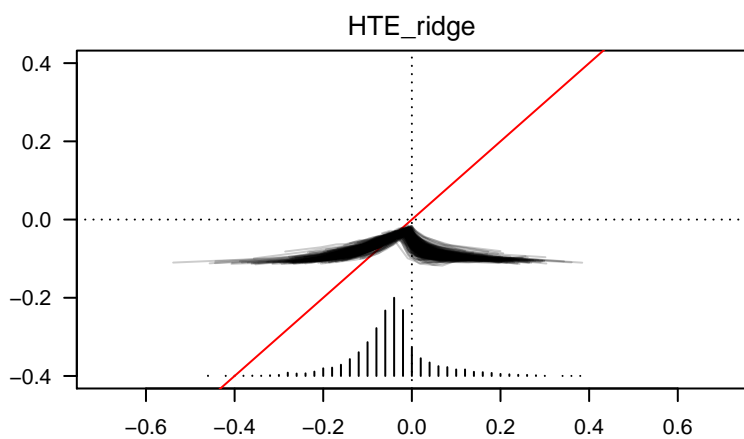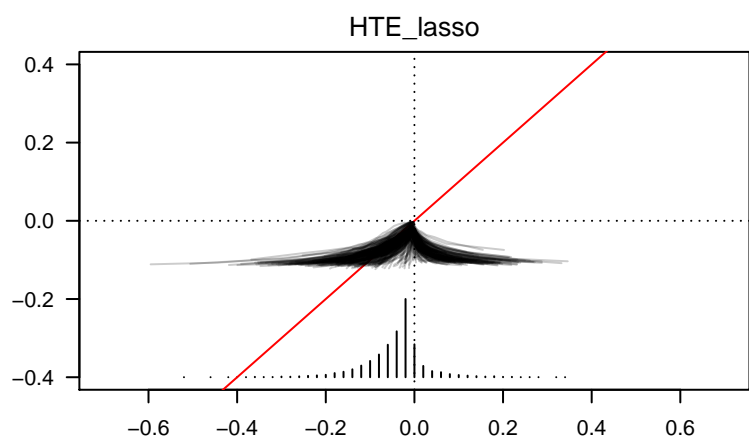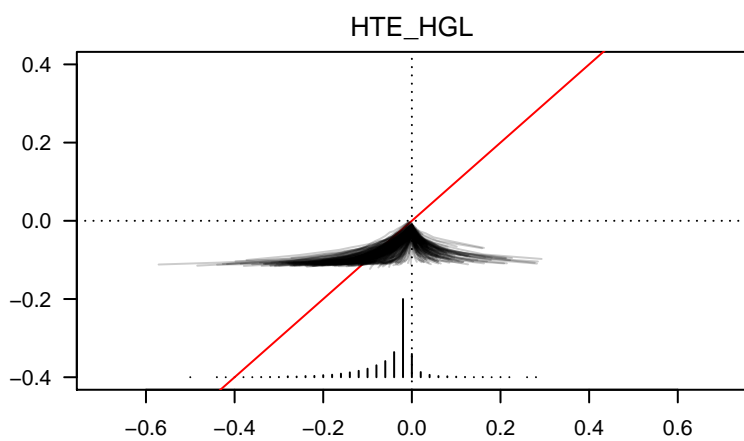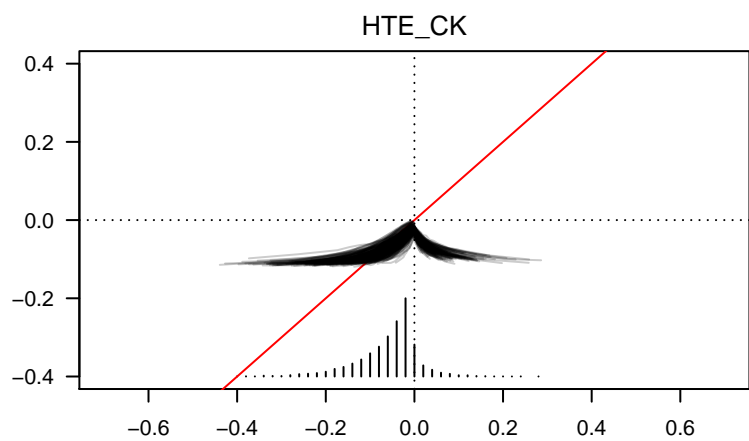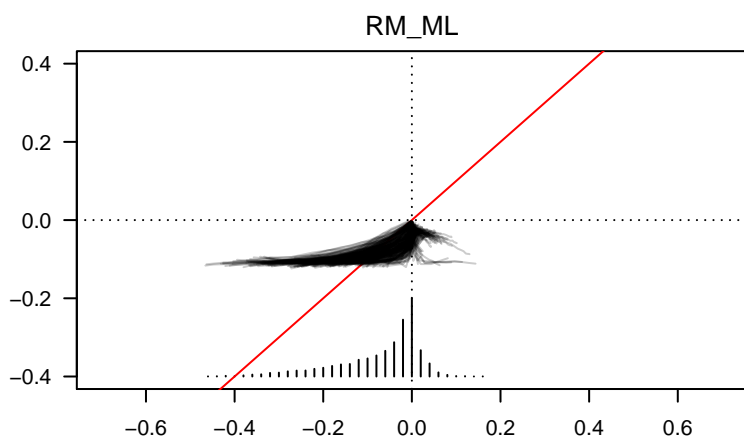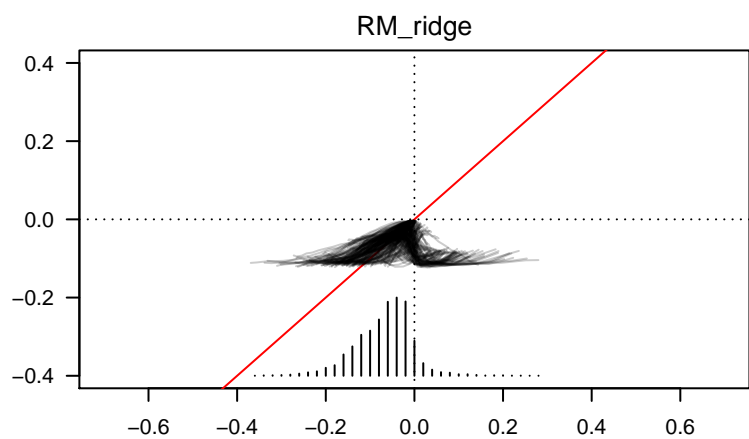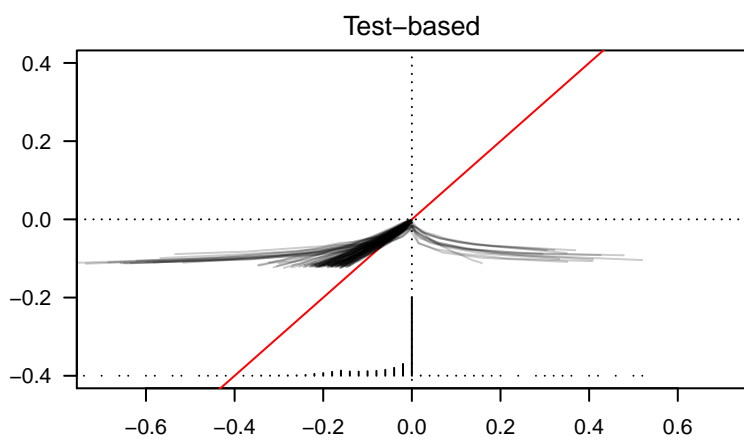

$\beta_t < 0$ , HOM, N=1200

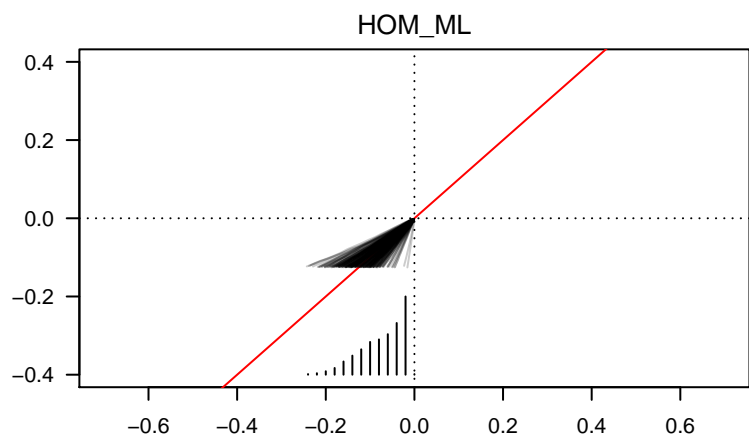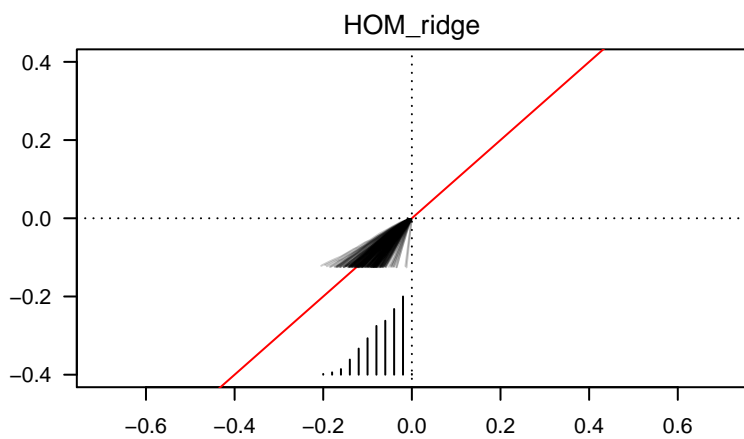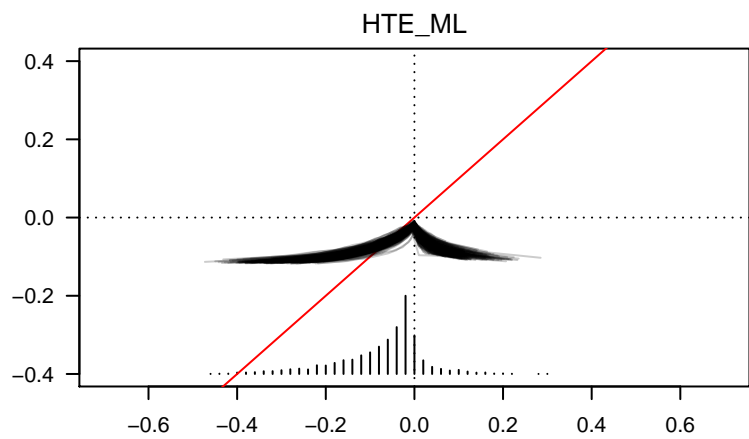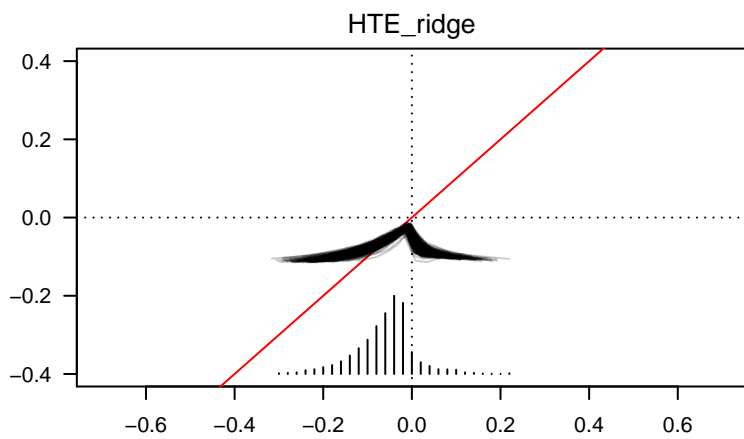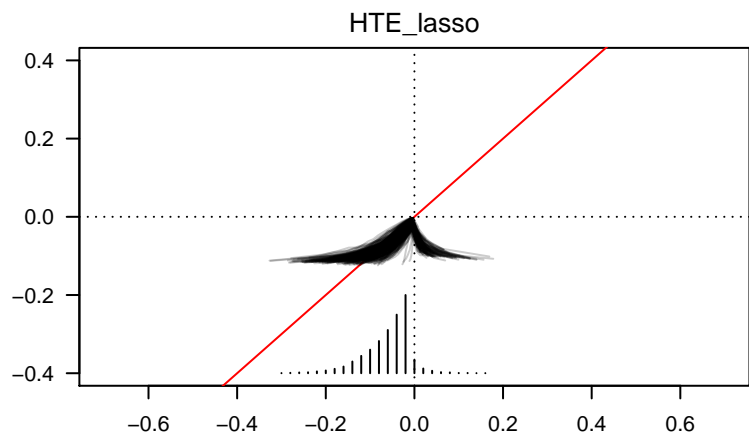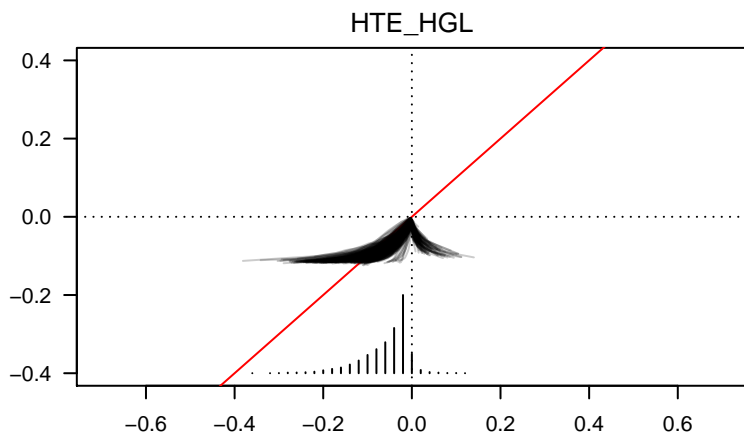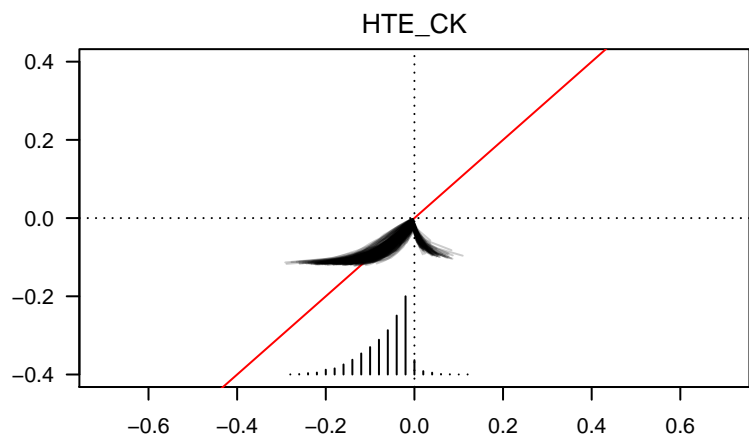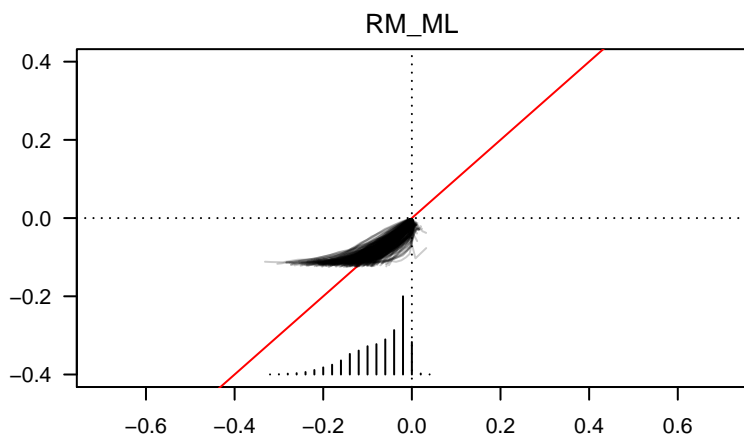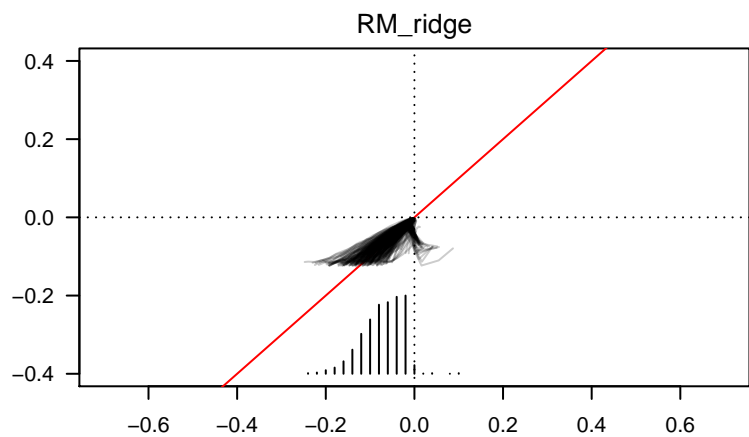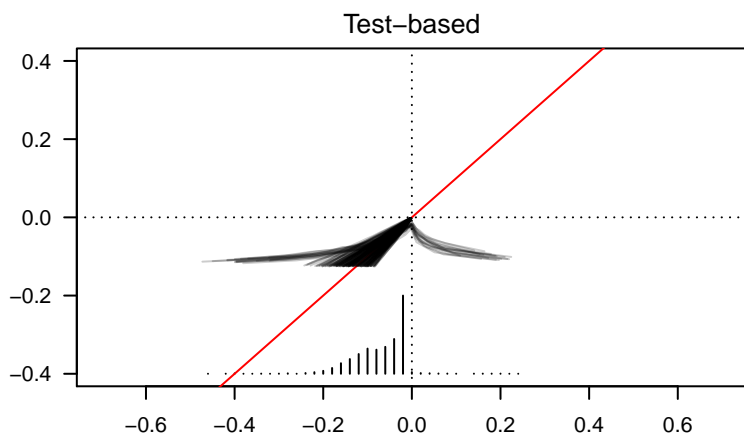

$\beta_t < 0$ , HOM, N=3600

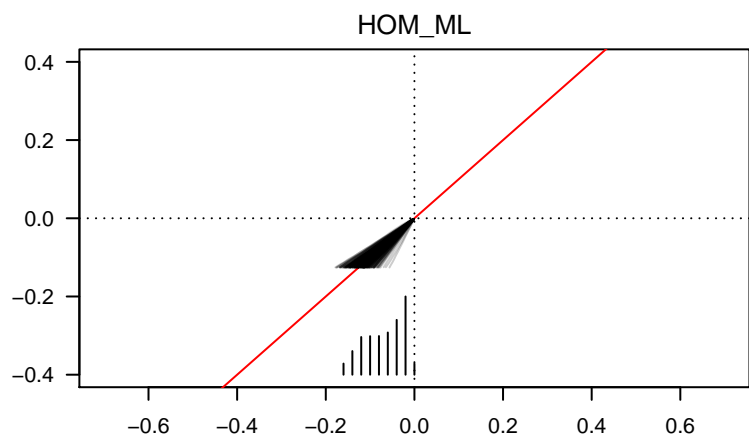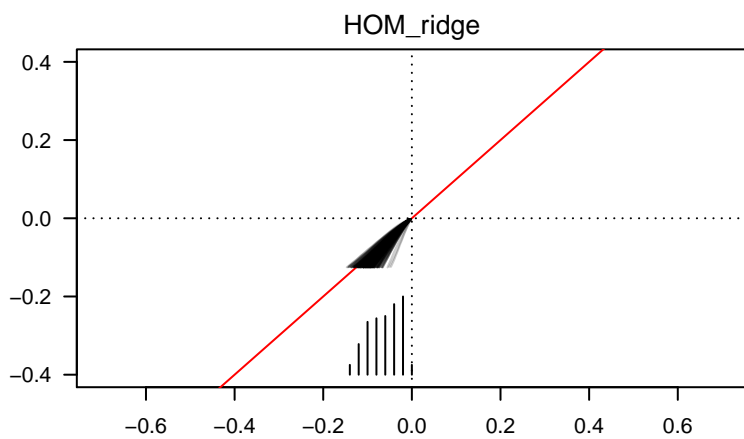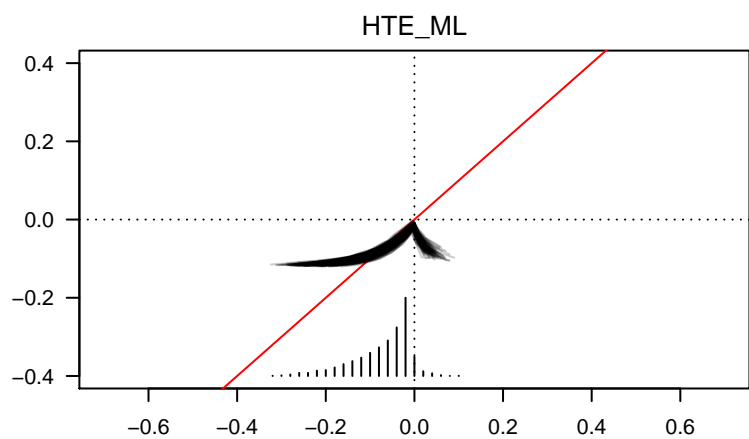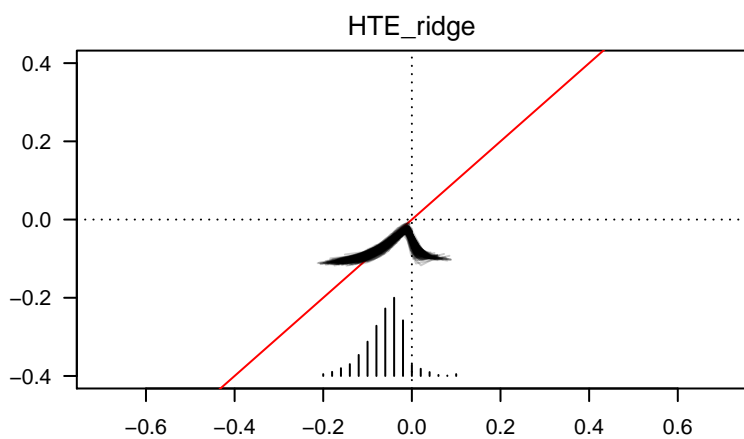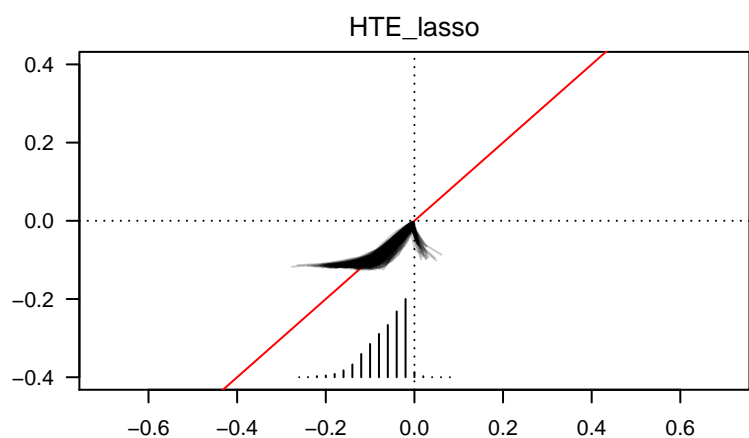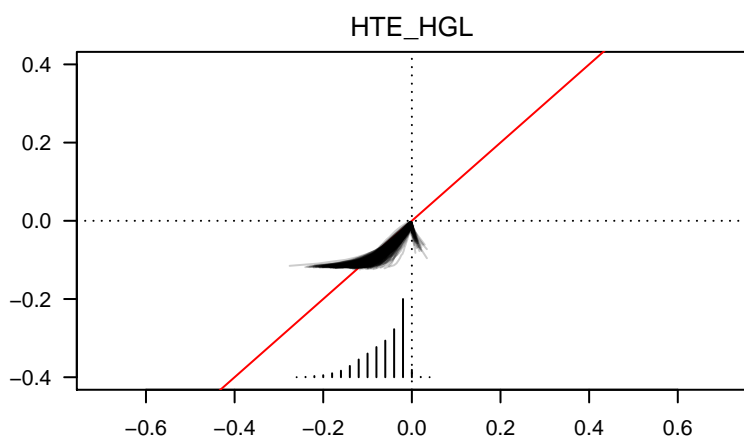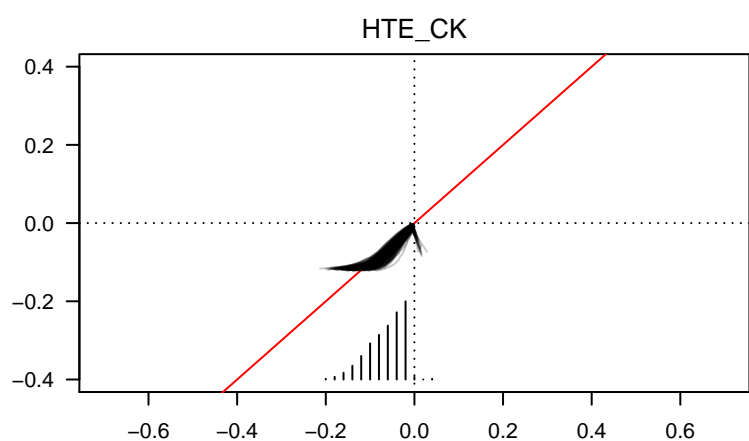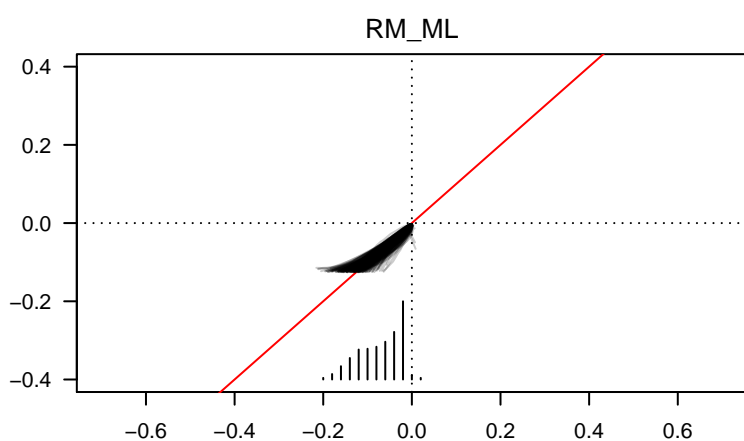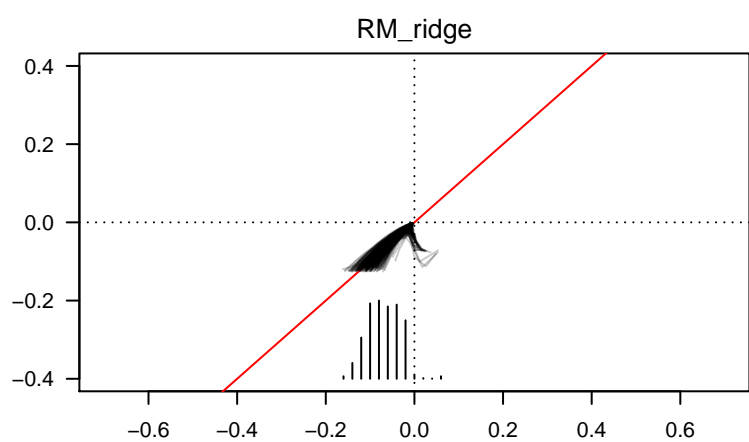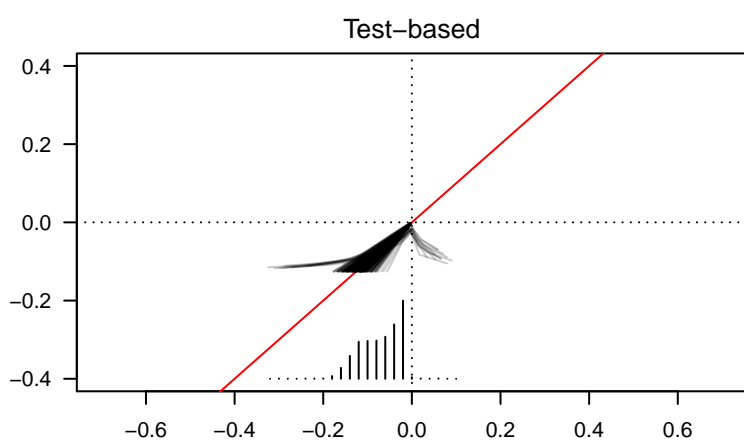

$\beta_t=0$ , HOM, N=400

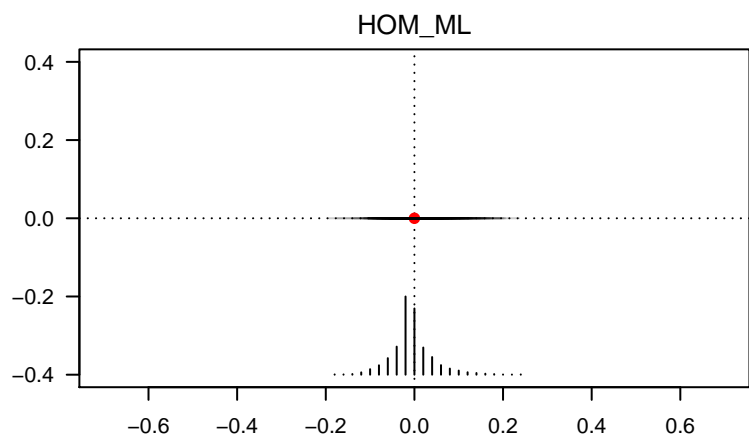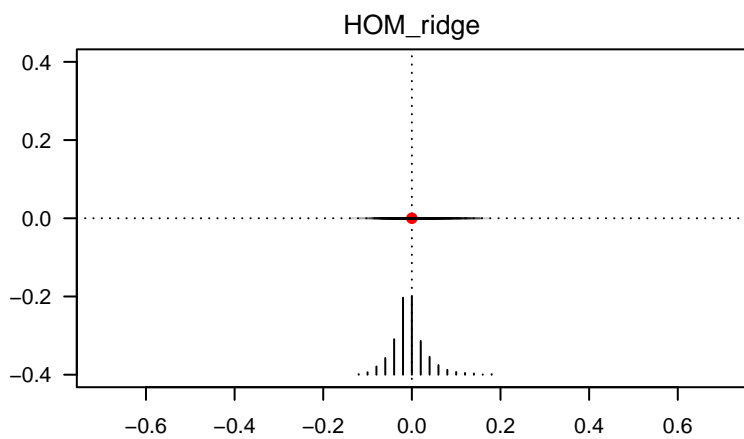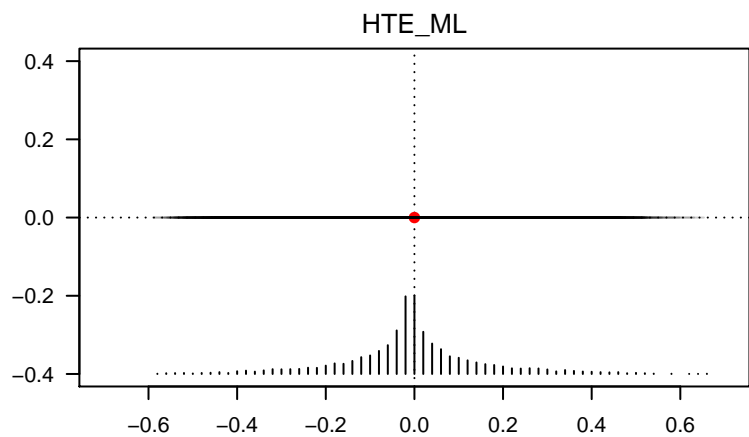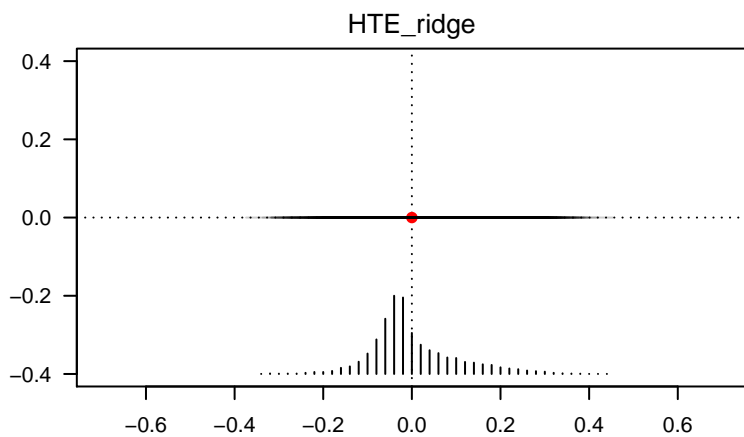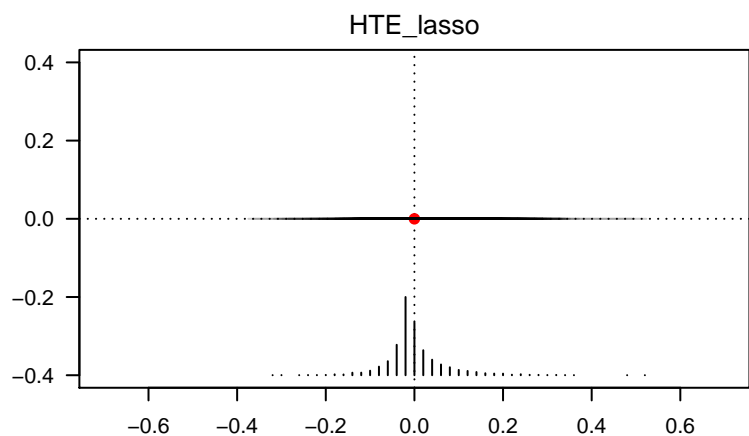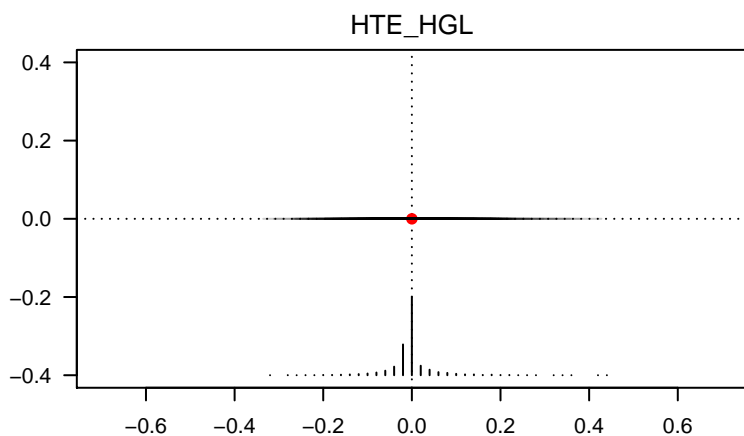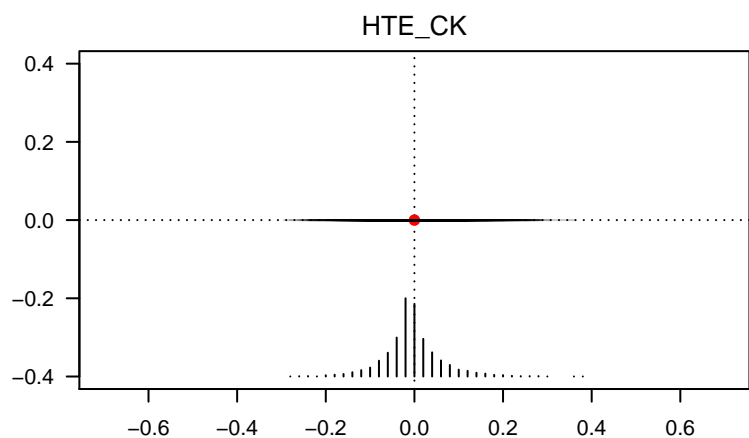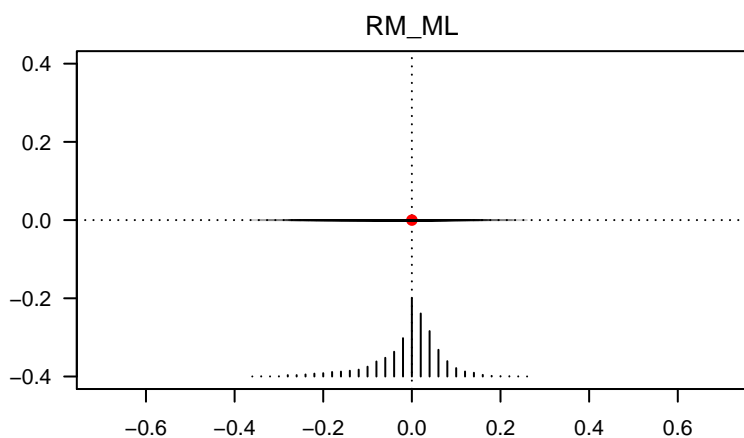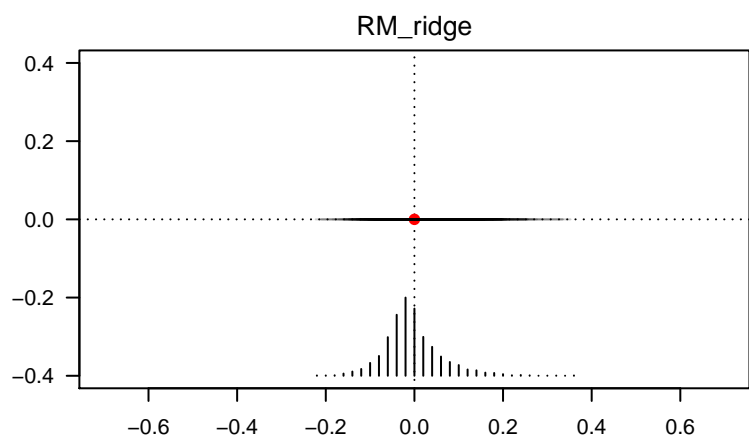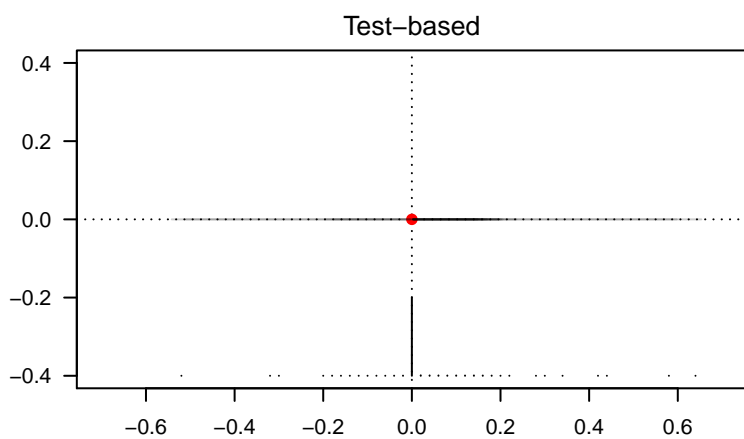

$\beta_t=0$ , HOM, N=1200

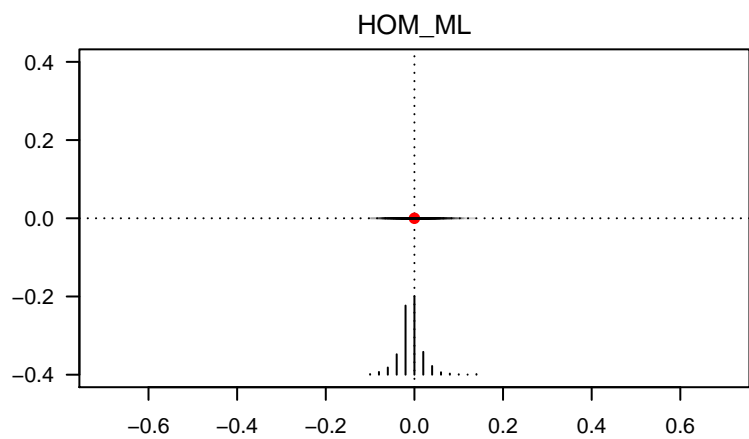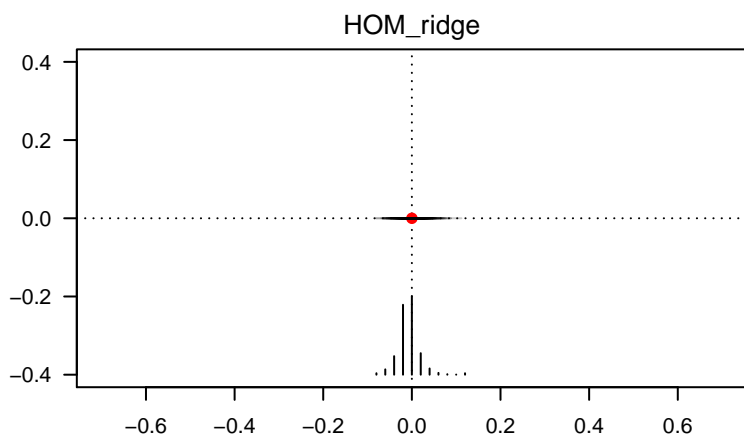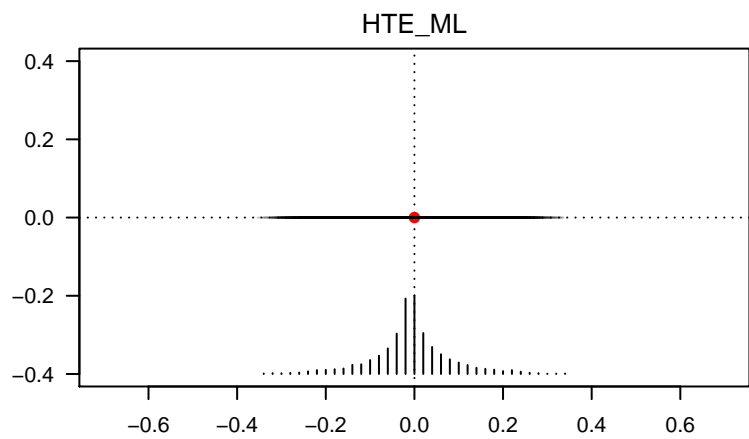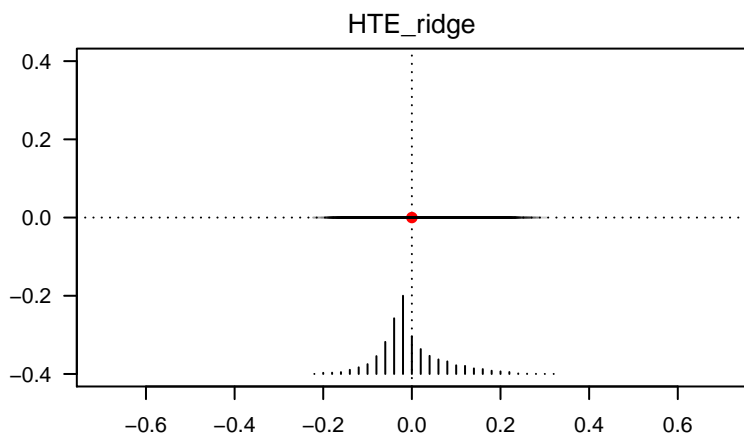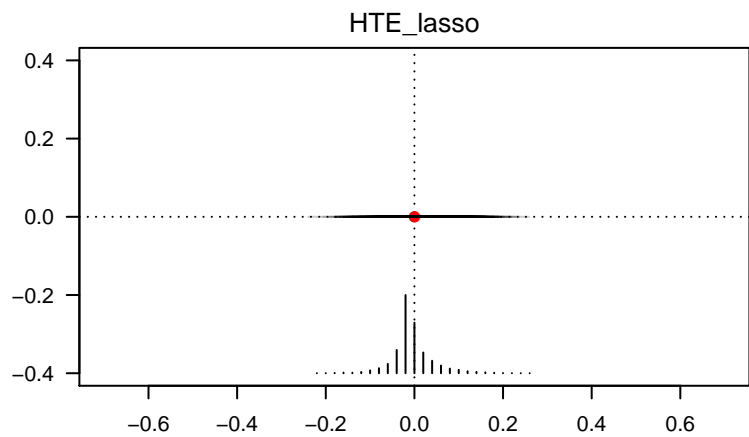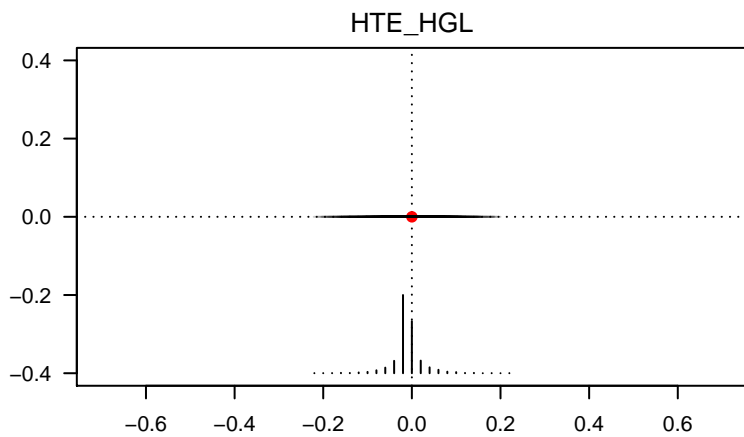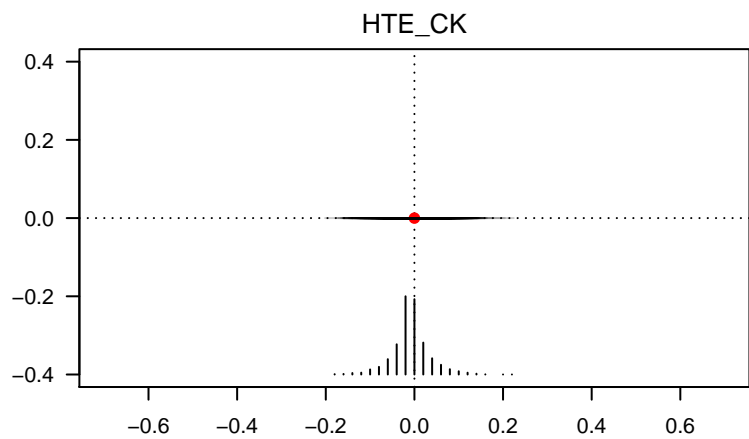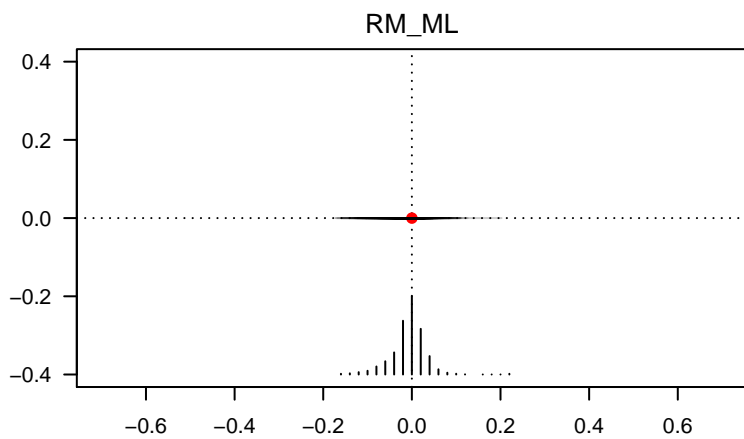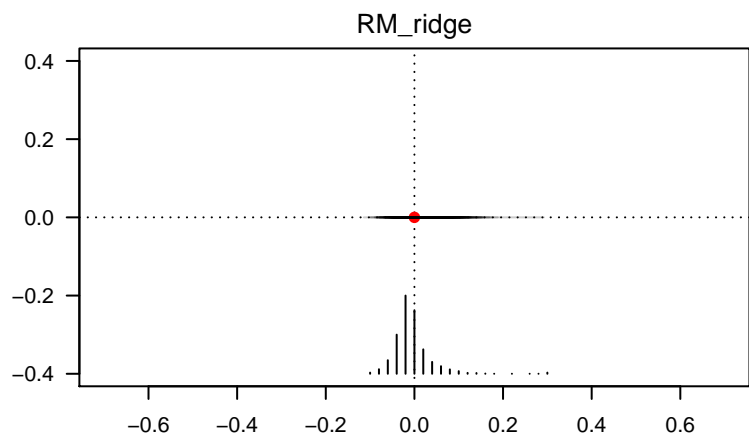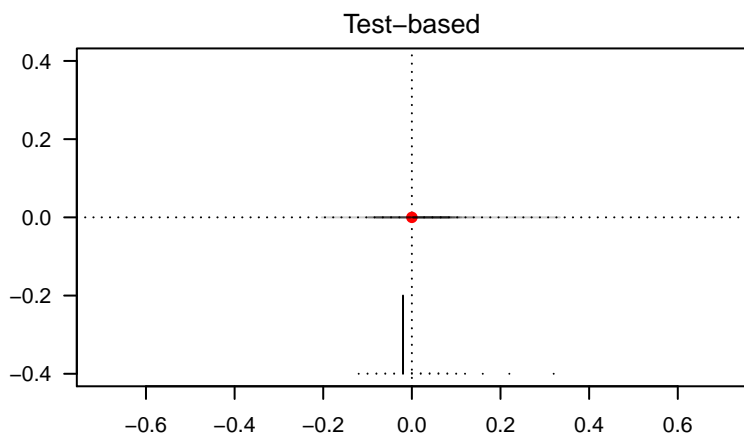

$\beta_t=0$ , HOM, N=3600

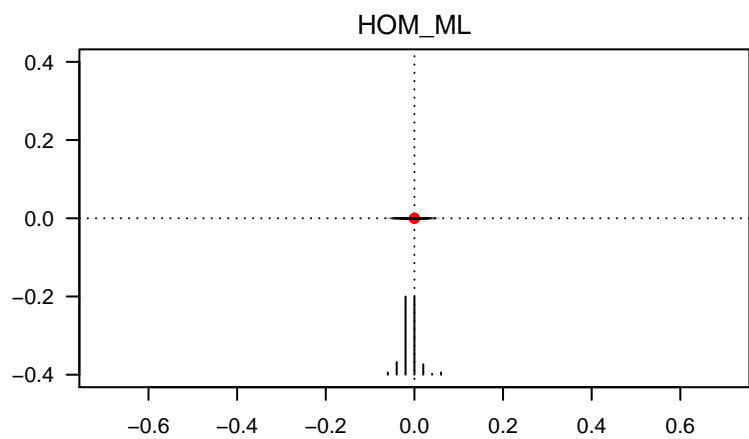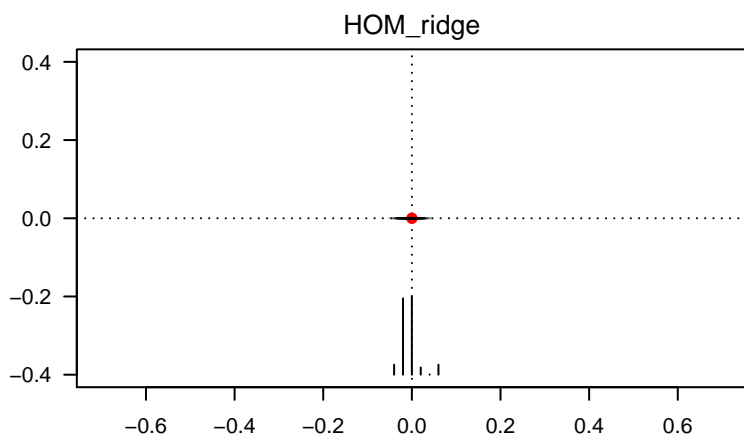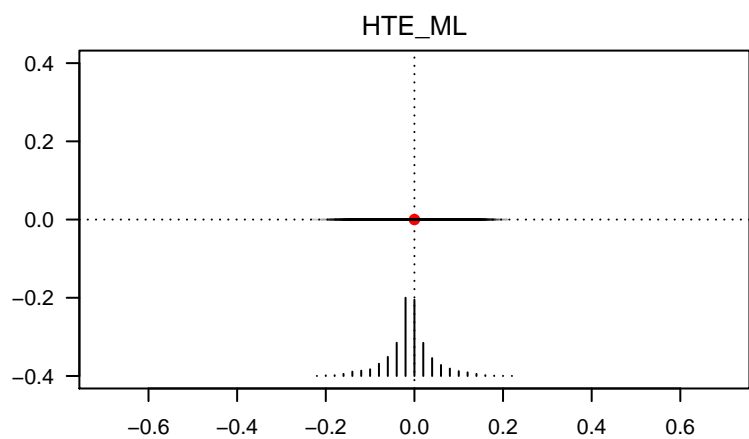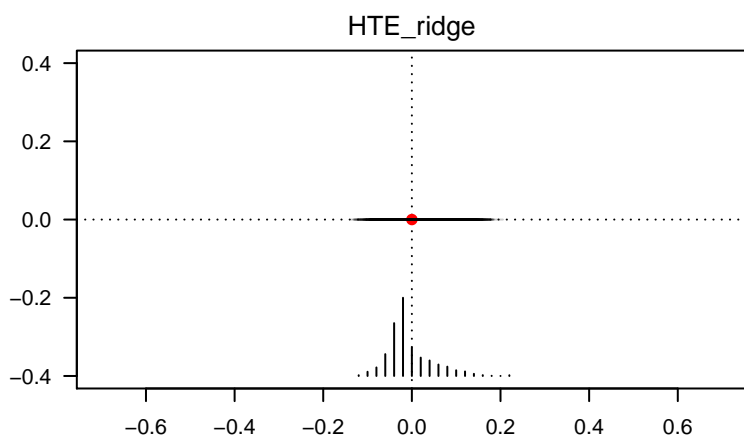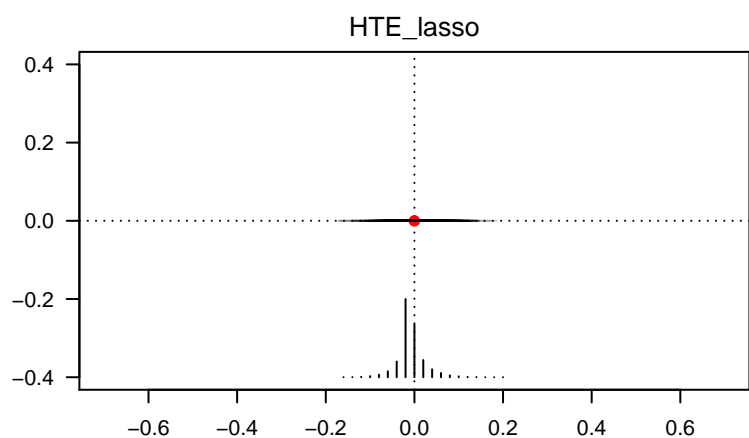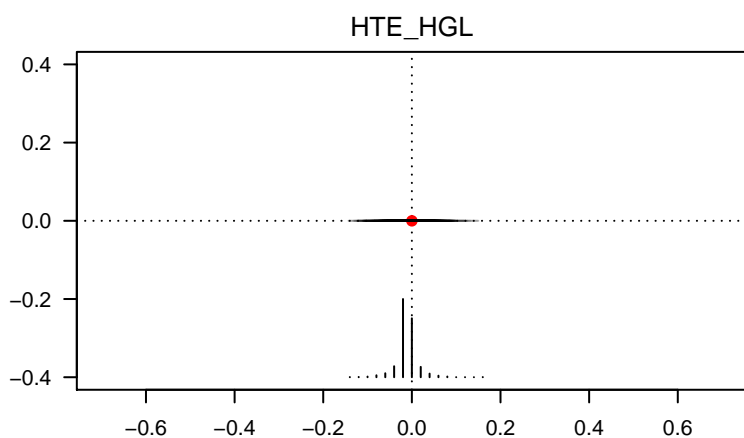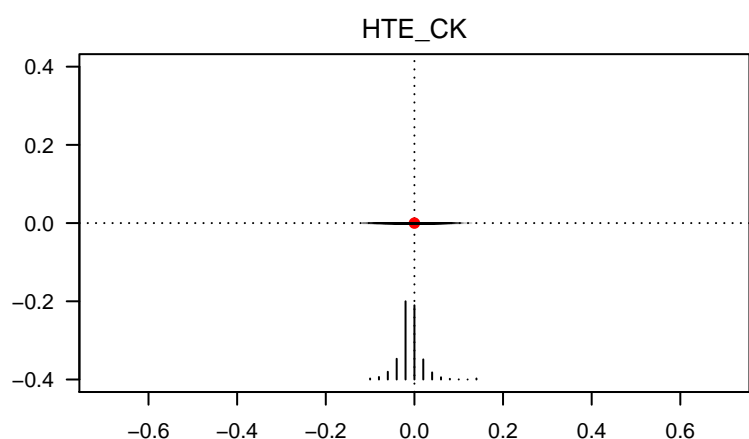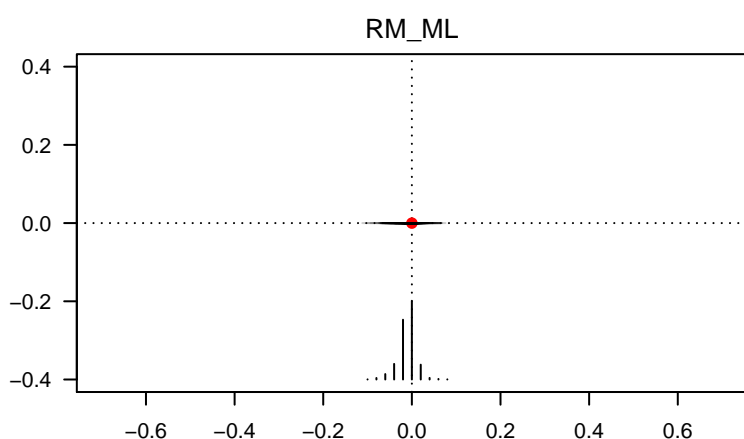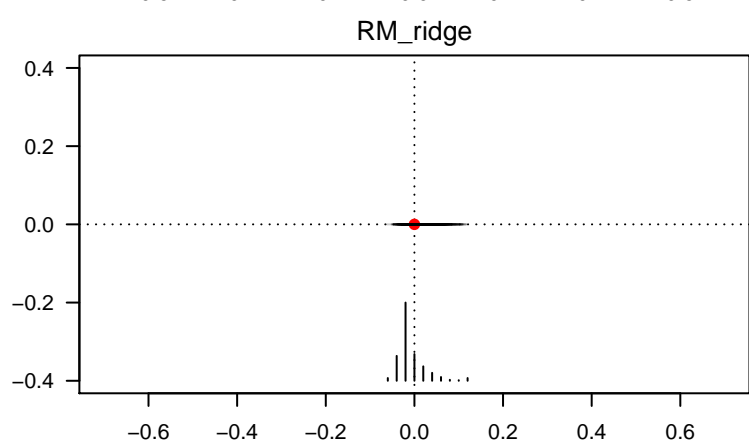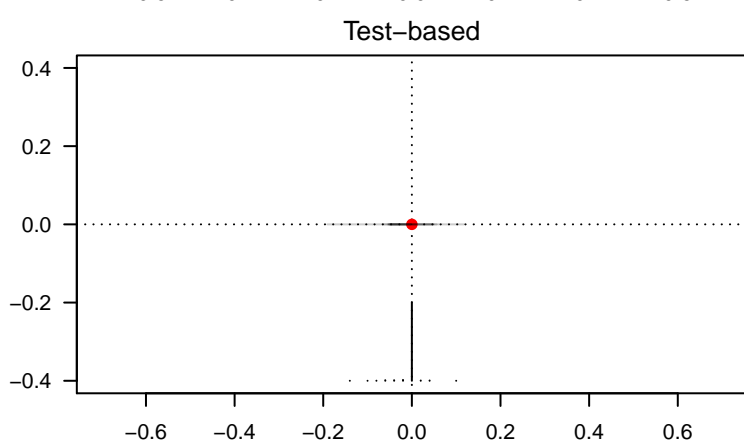

$\beta_t < 0$ , HTE,  $N=400$ 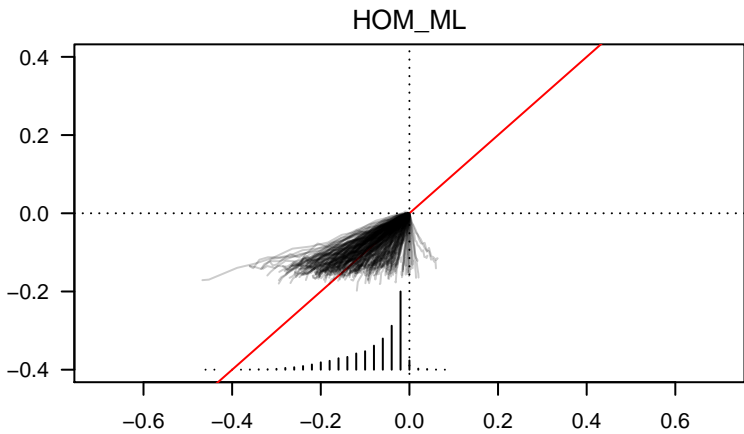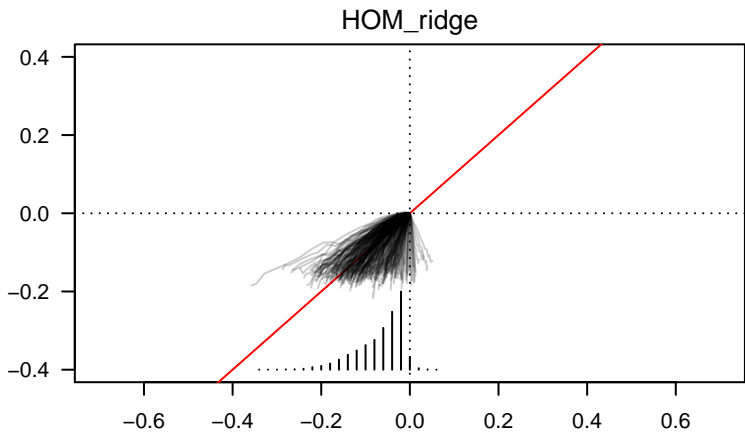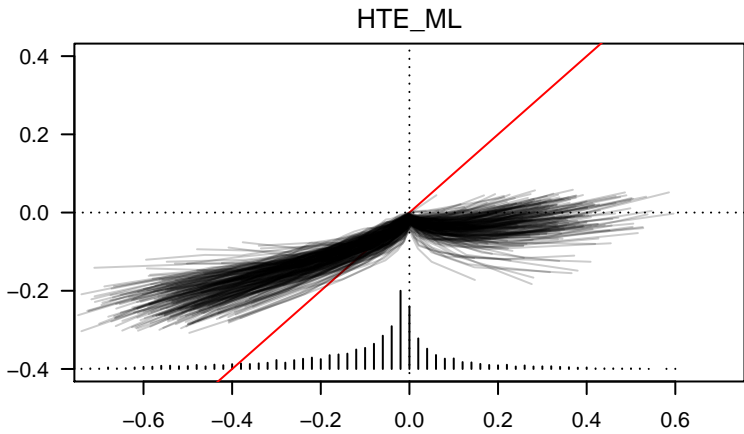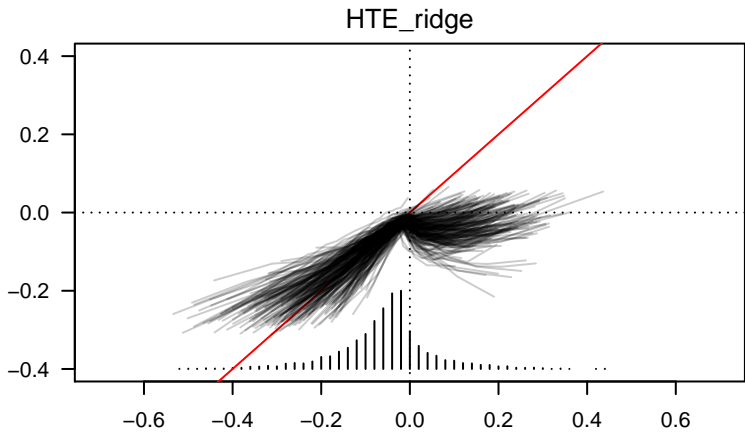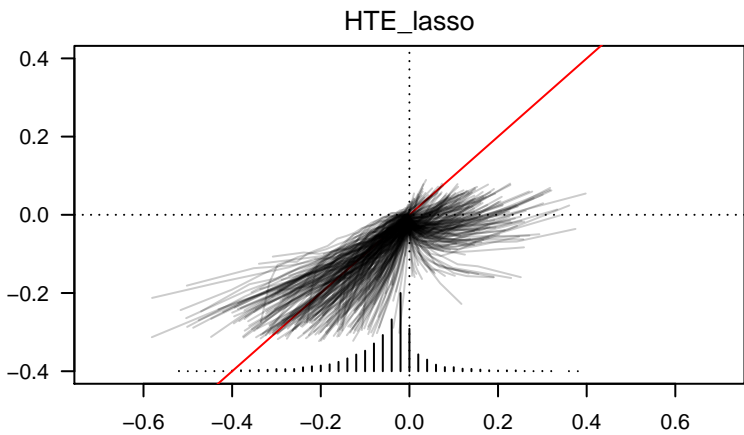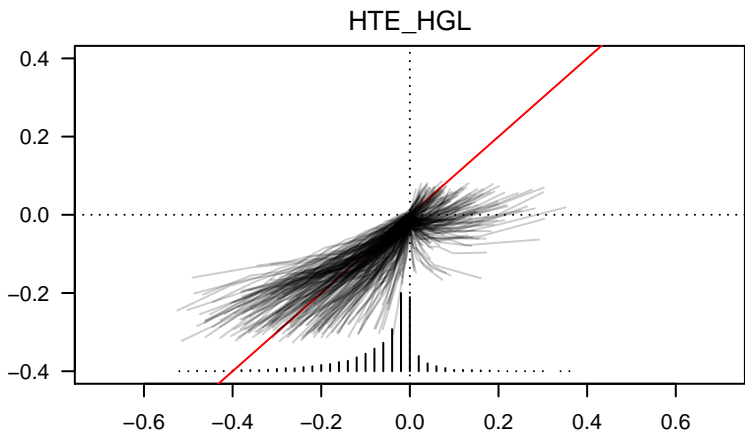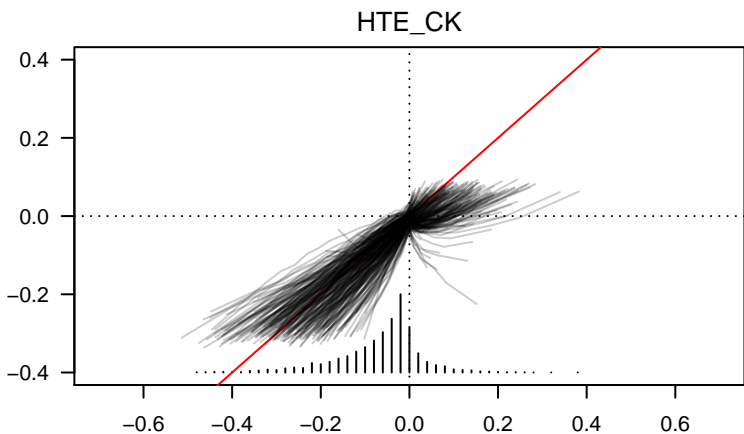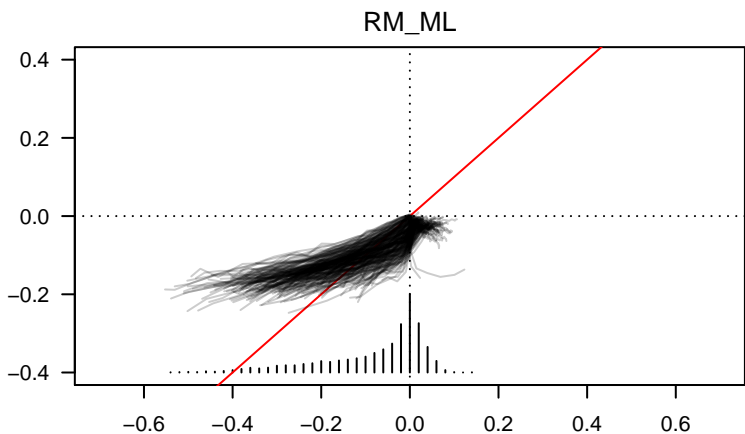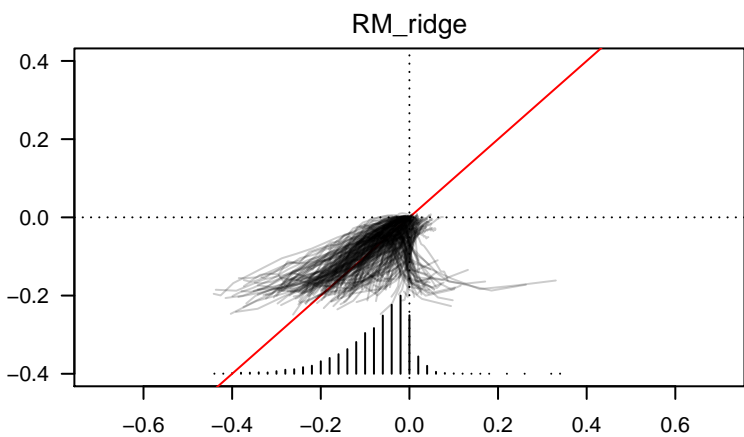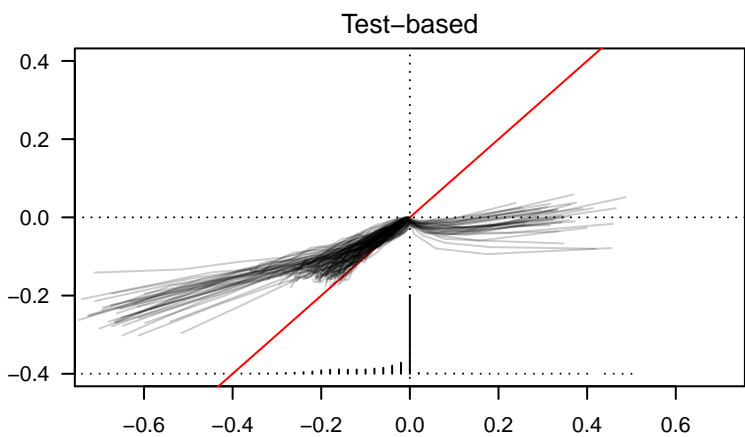

$\beta_t < 0$ , HTE, N=1200

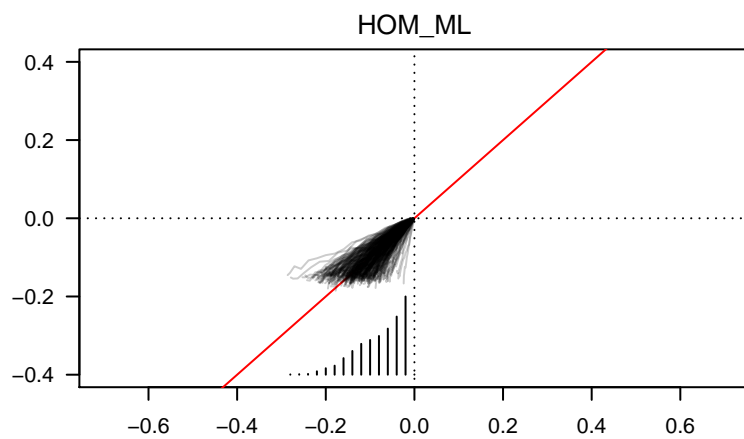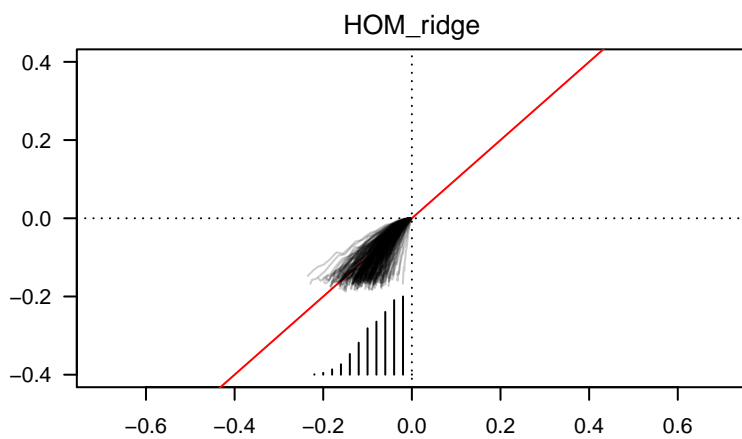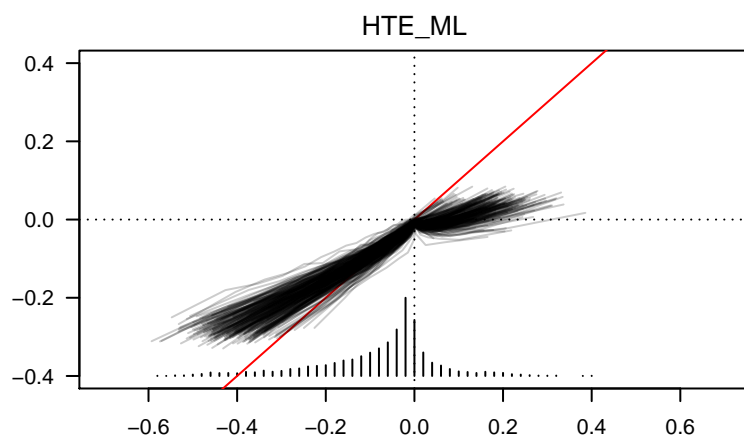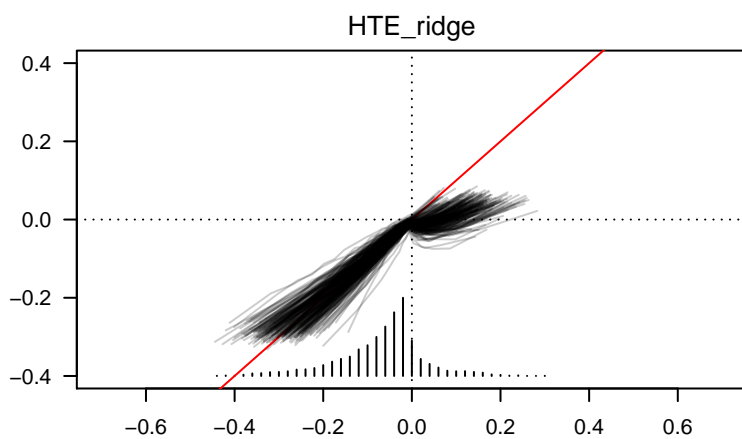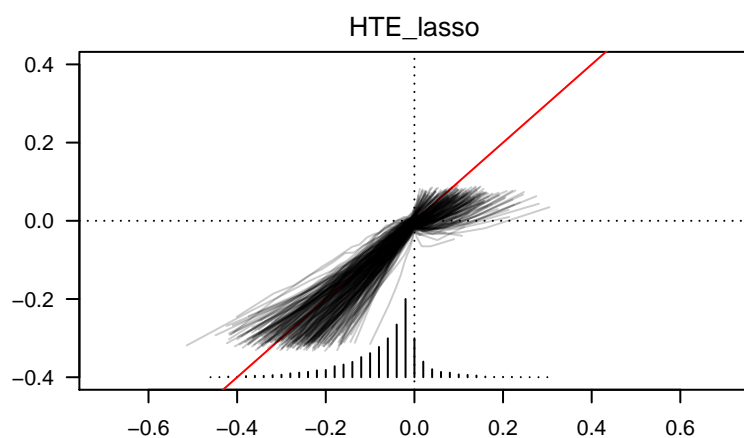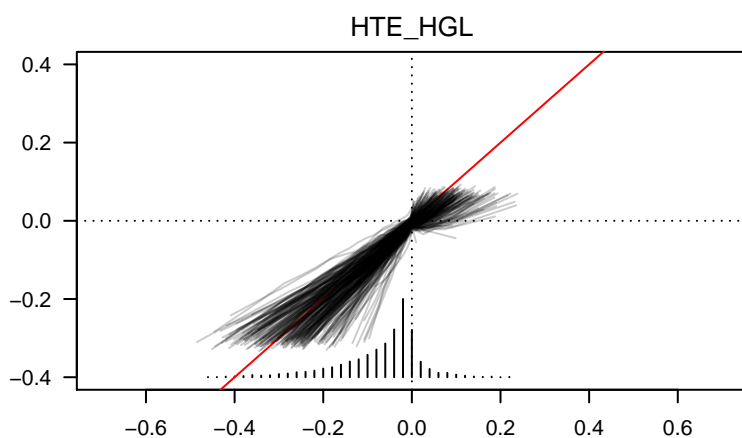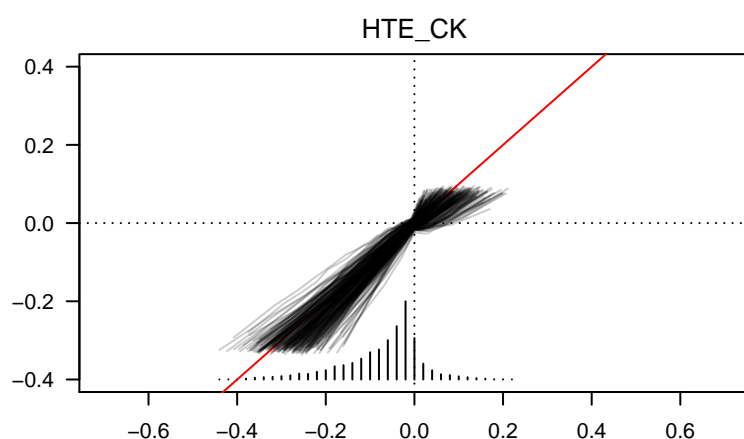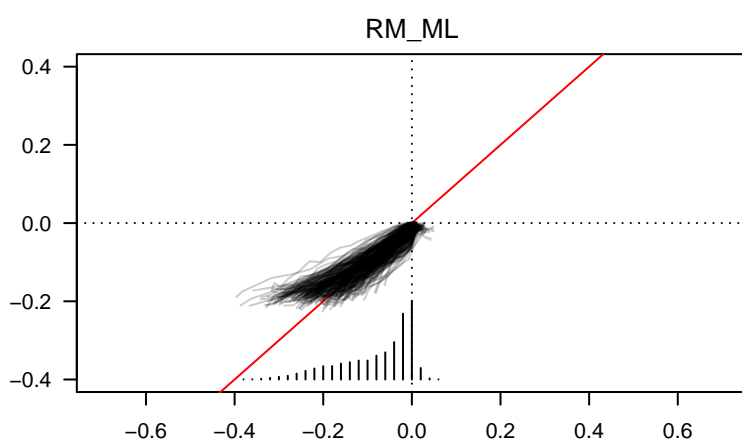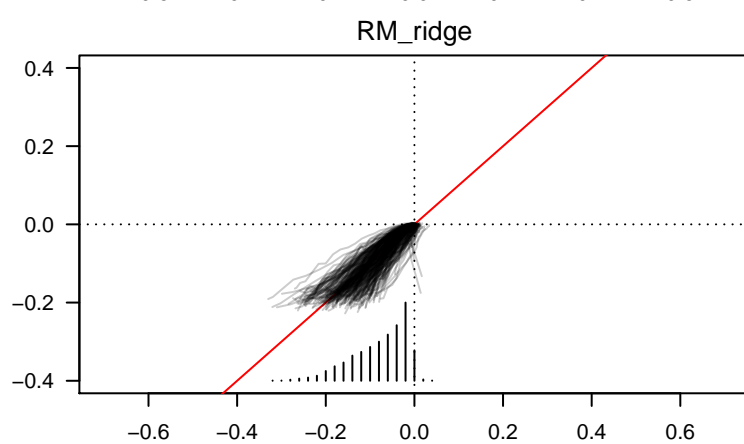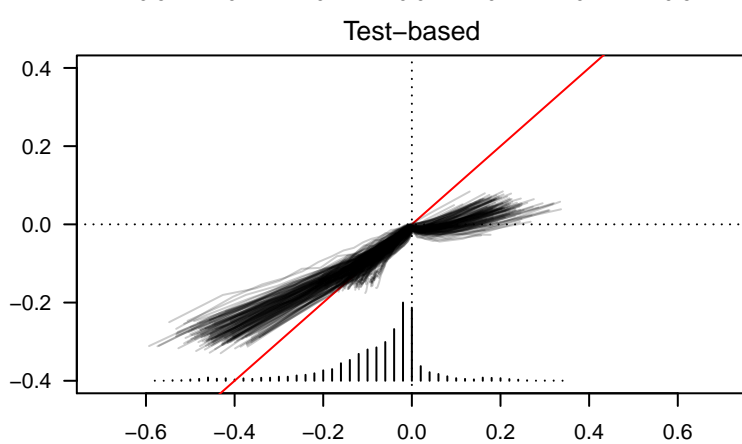



$\beta_t < 0$ , HTE, N=3600

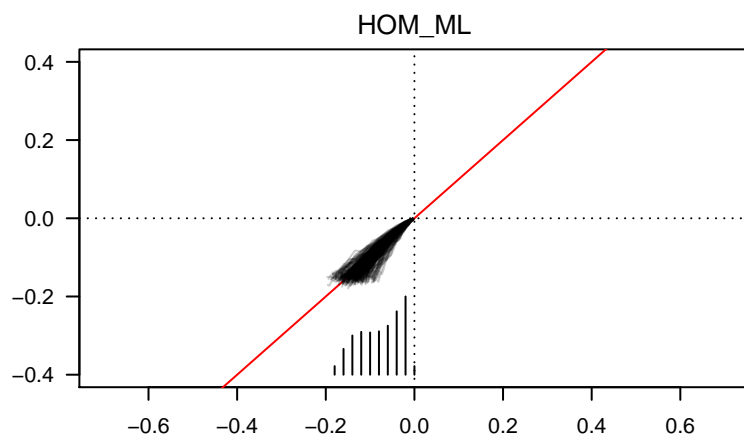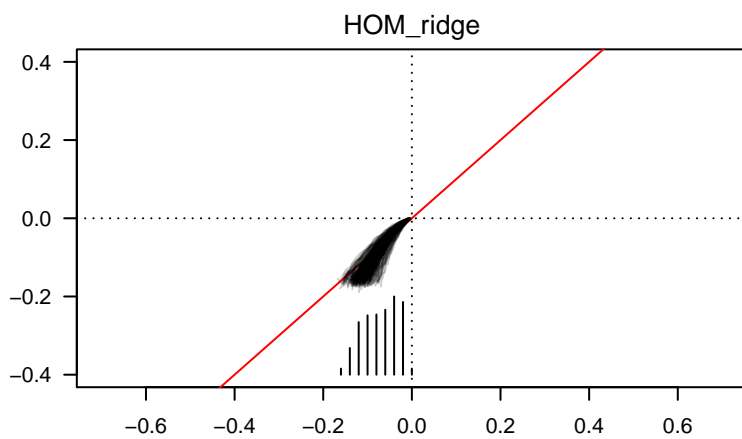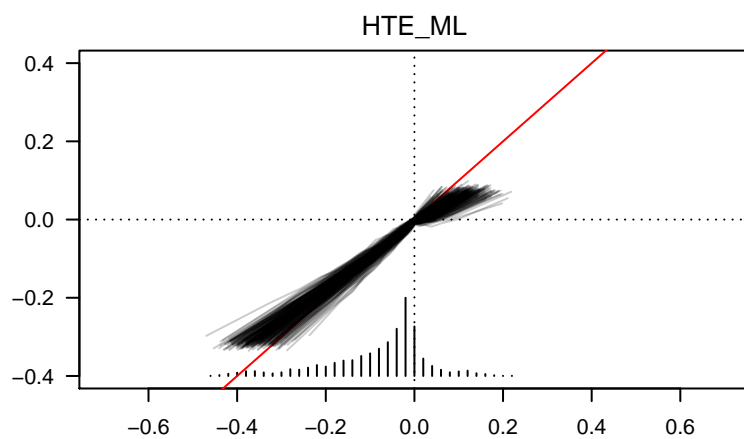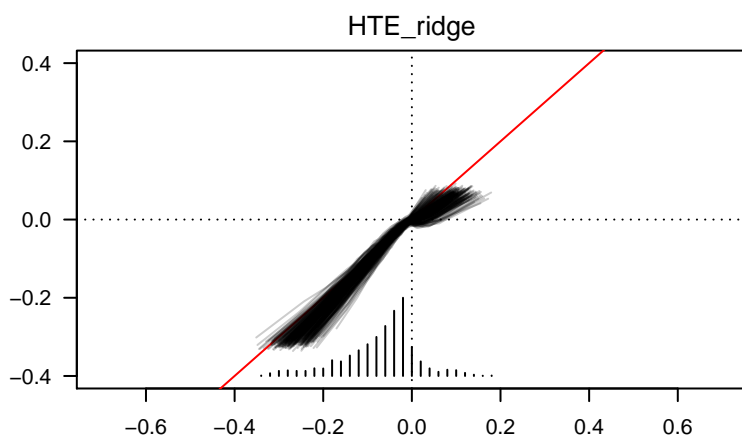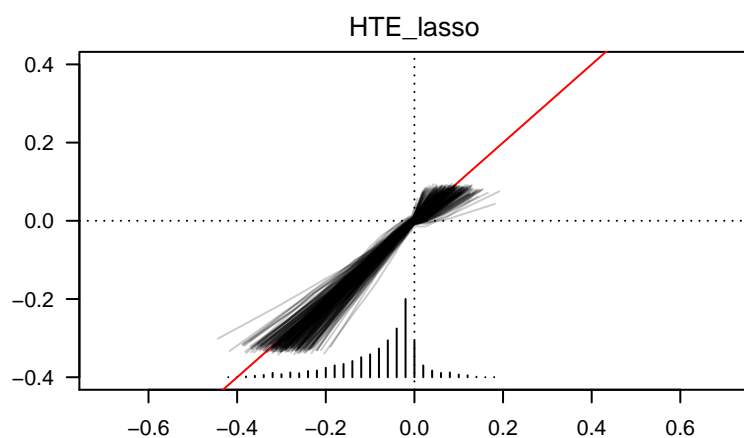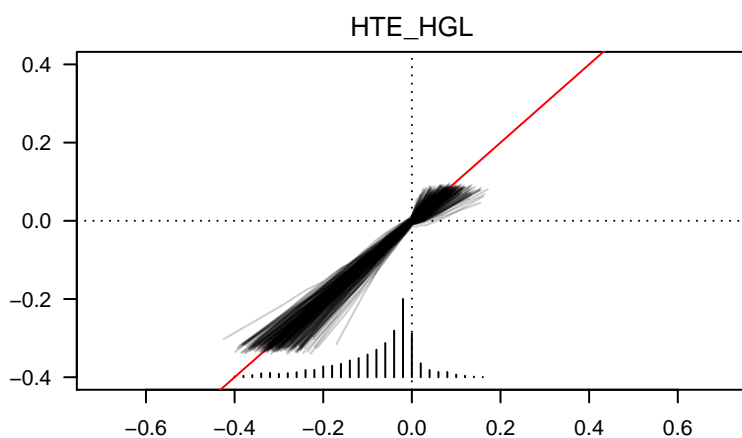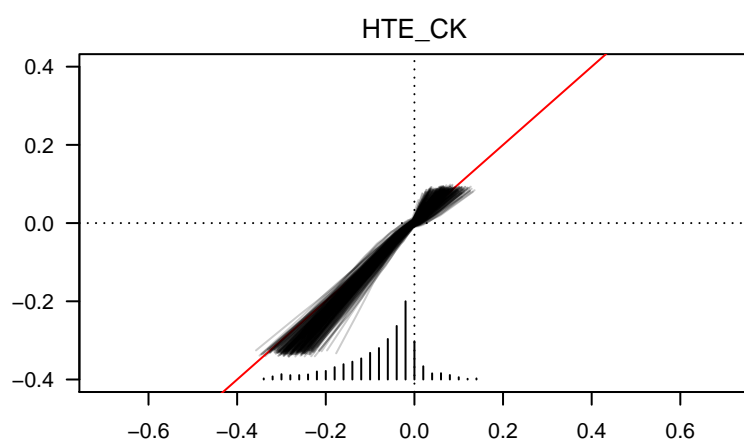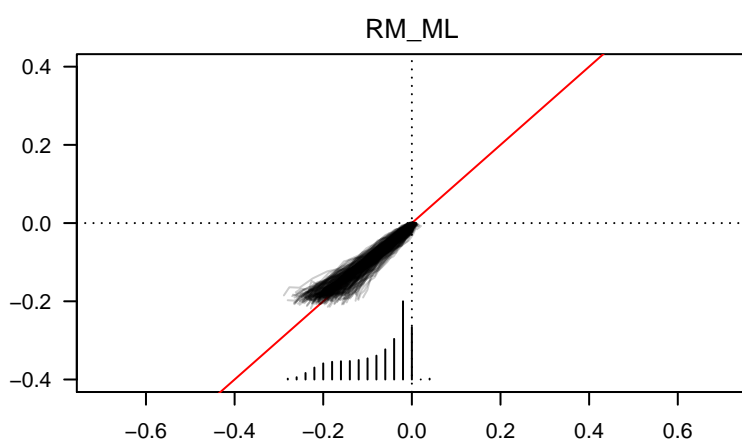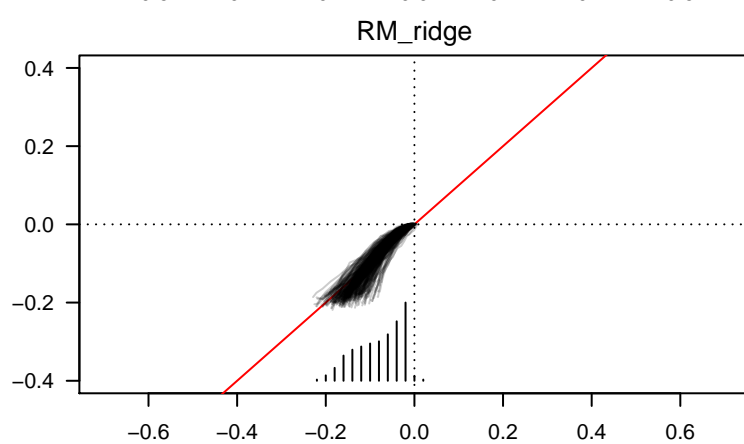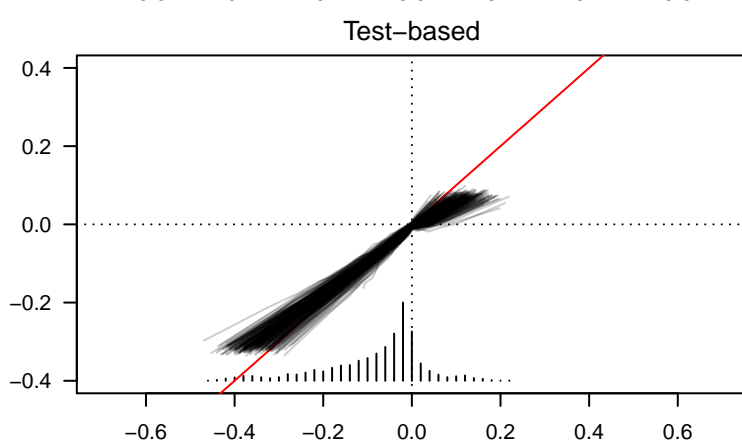

$\beta_t=0$ , HTE, N=400

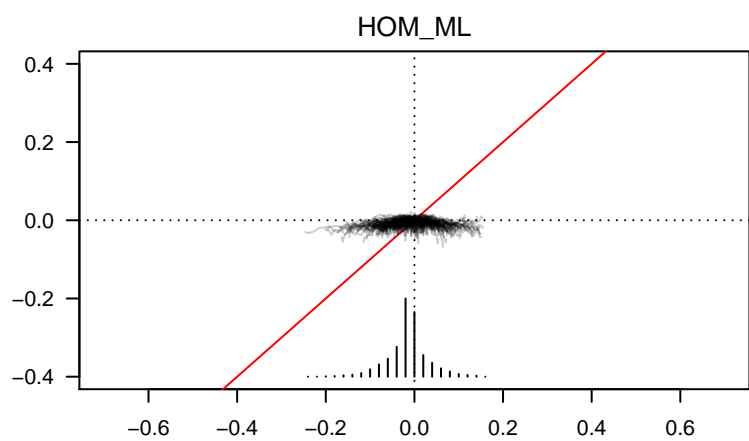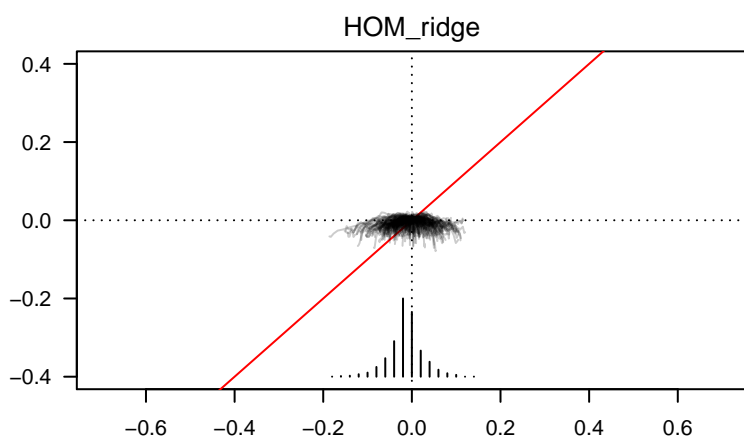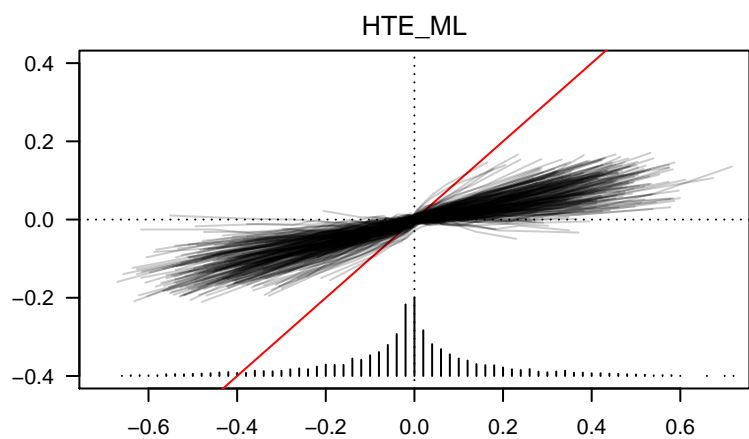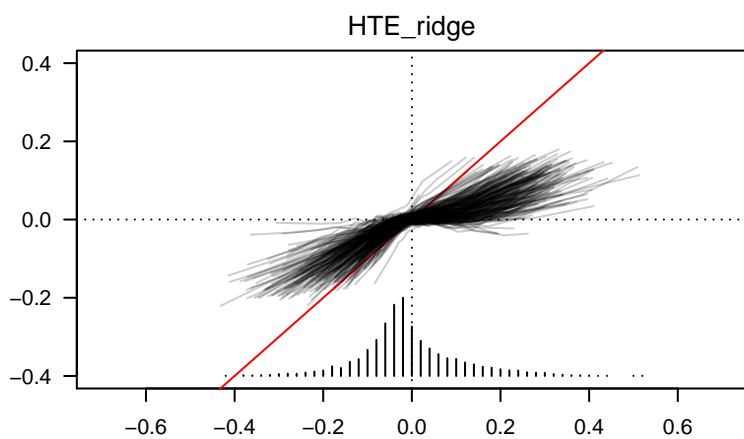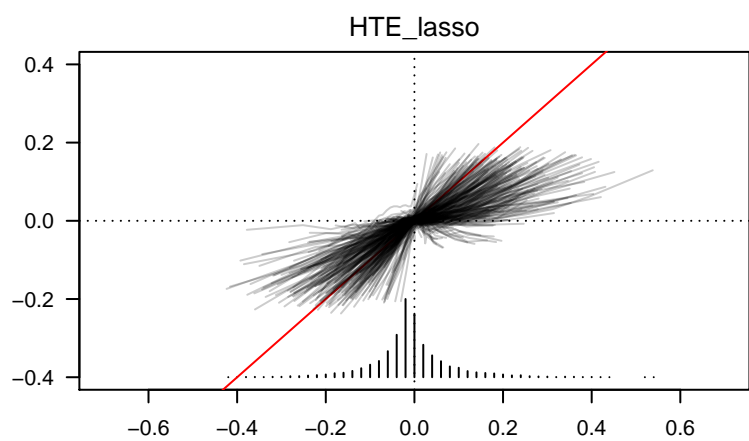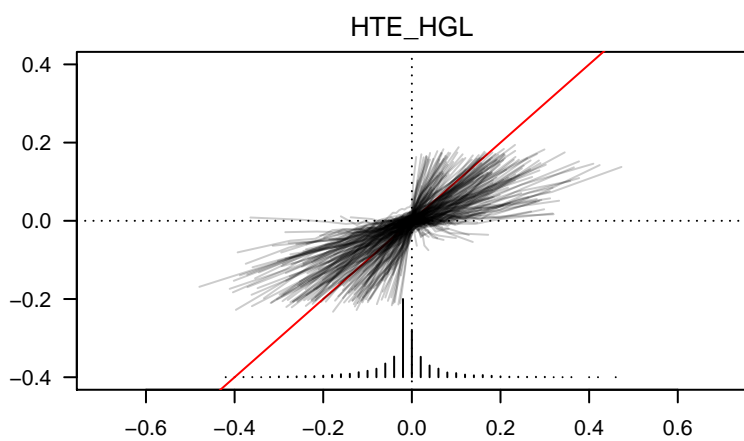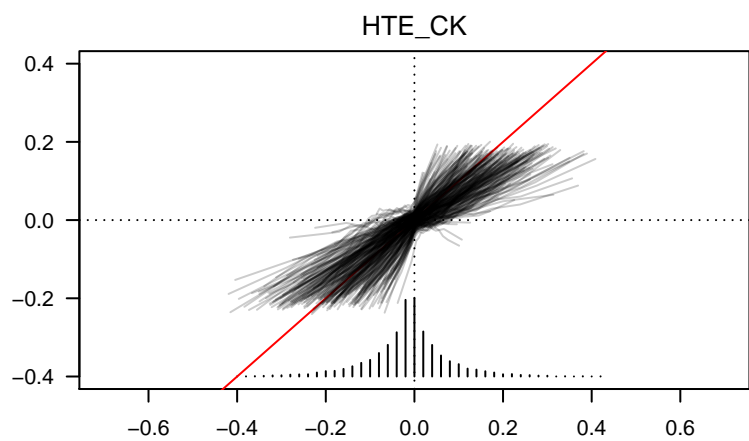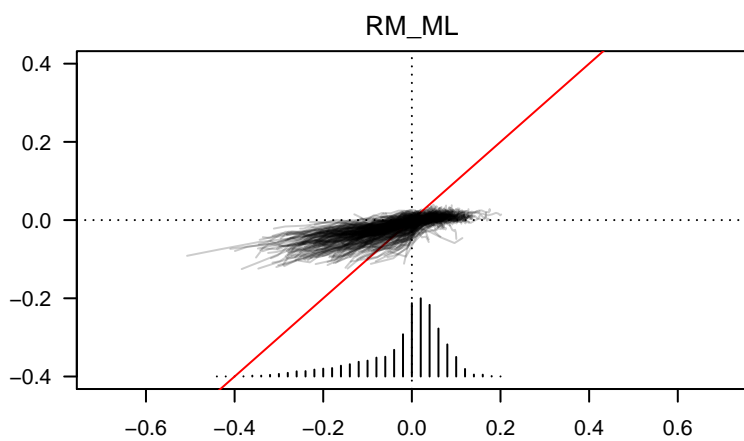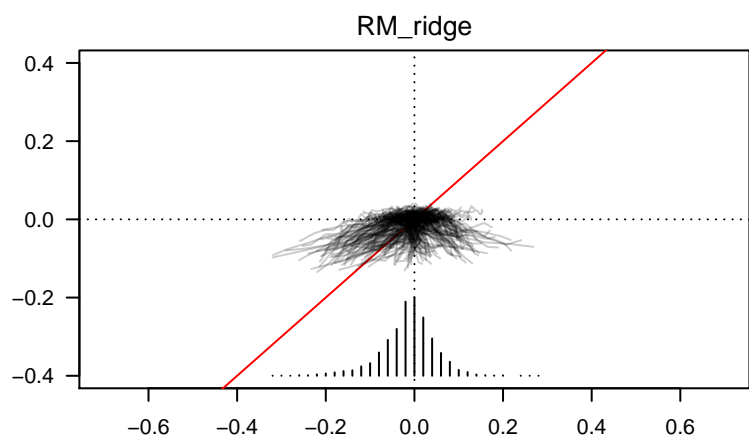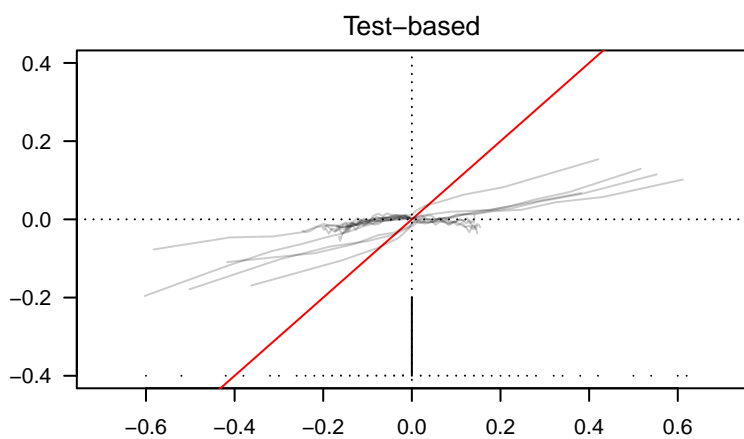

$\beta_t=0$ , HTE, N=1200

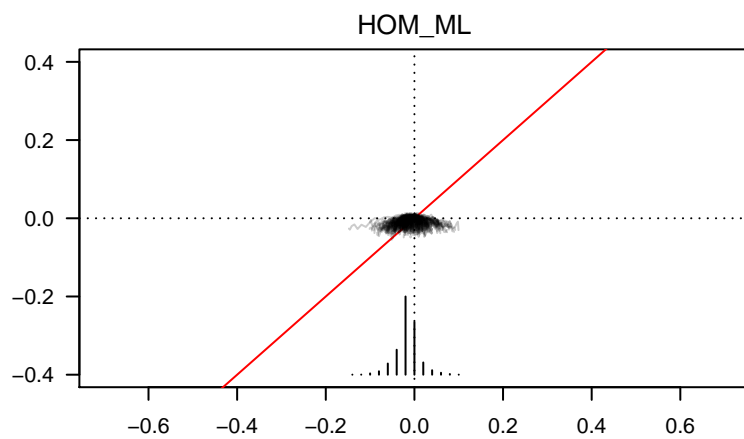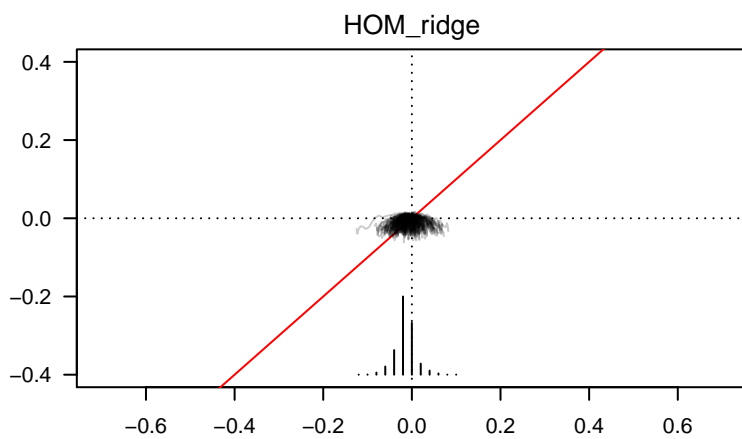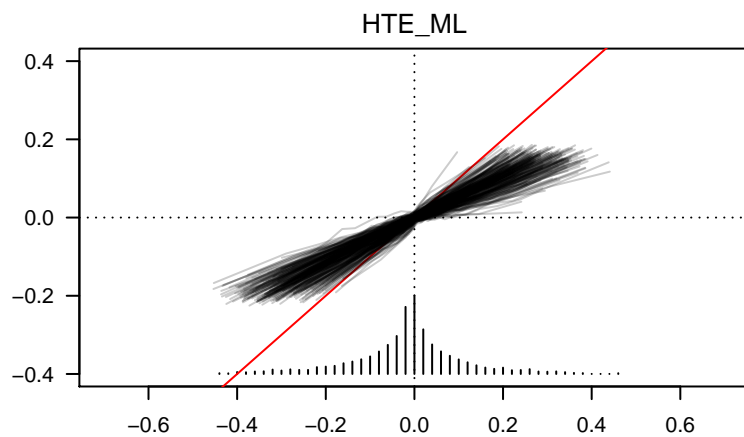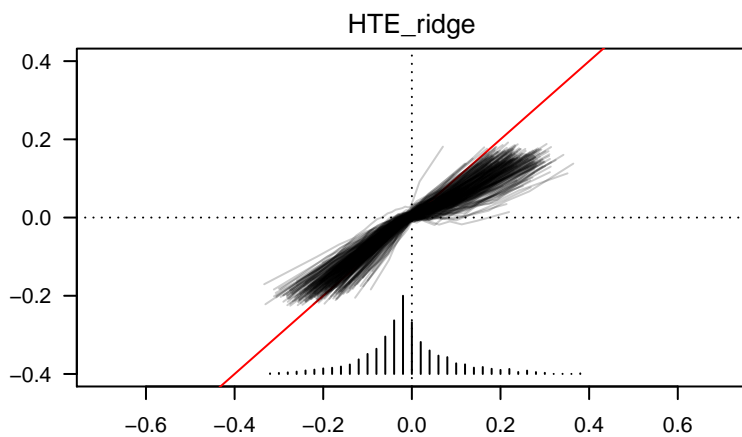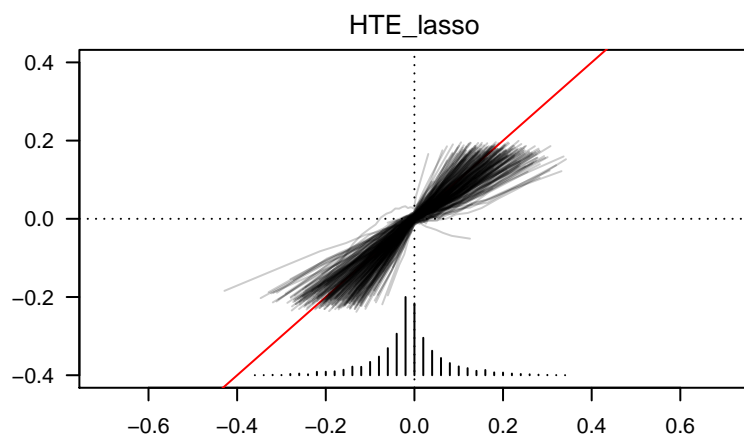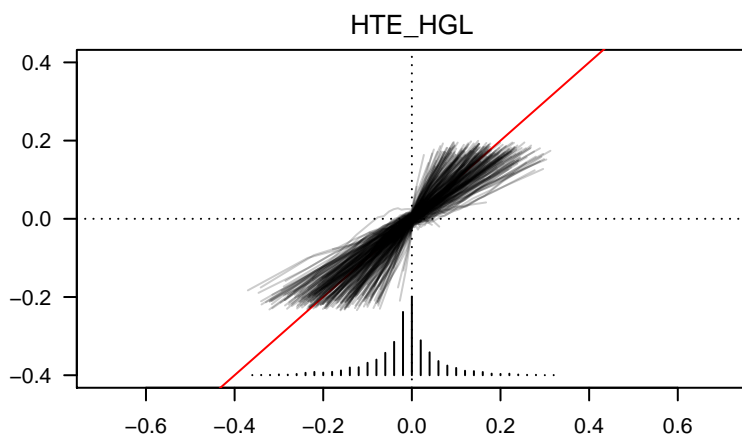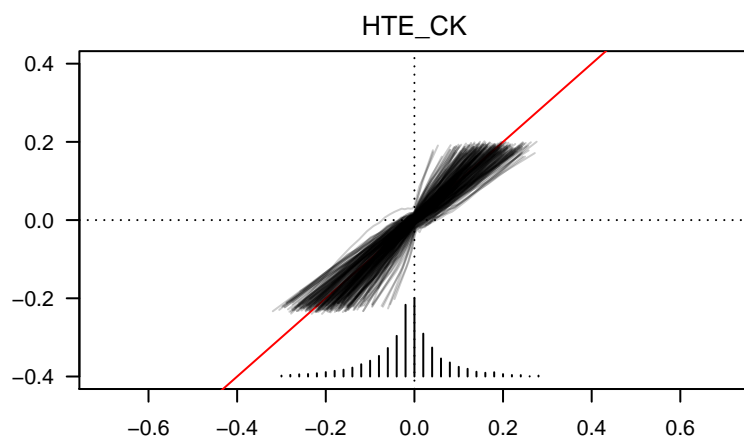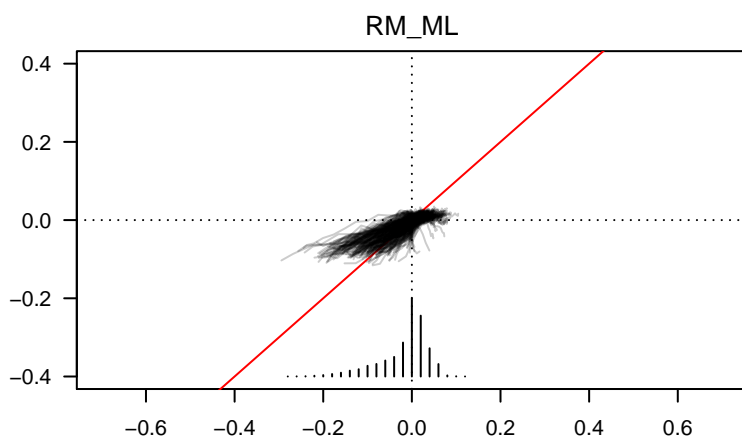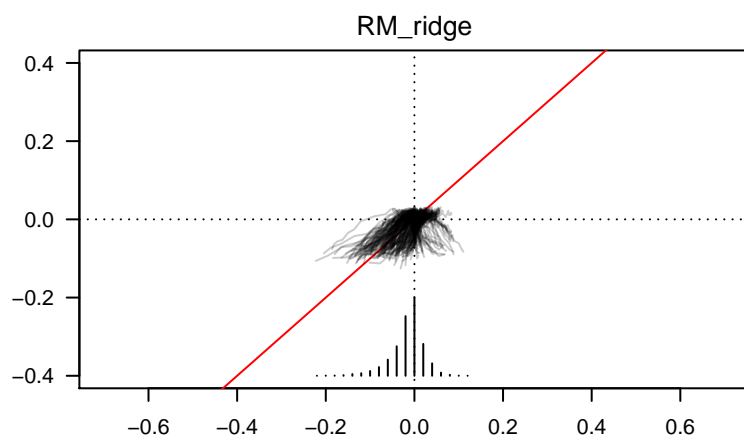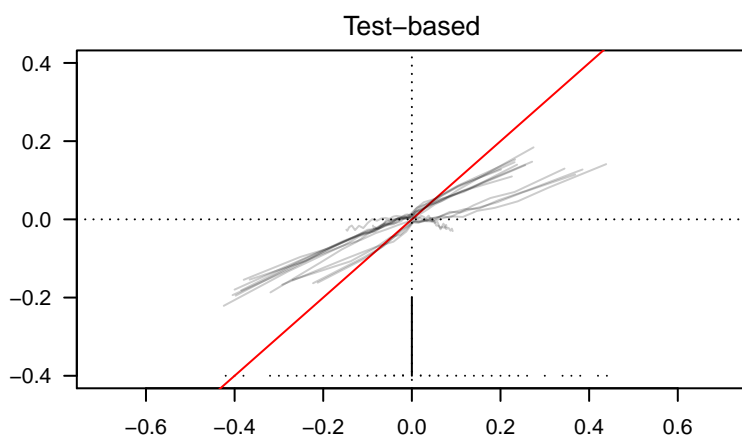

$\beta_t=0$ , HTE, N=3600

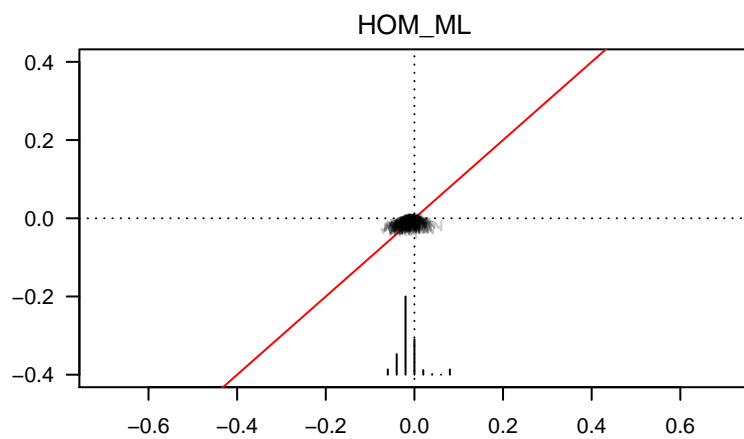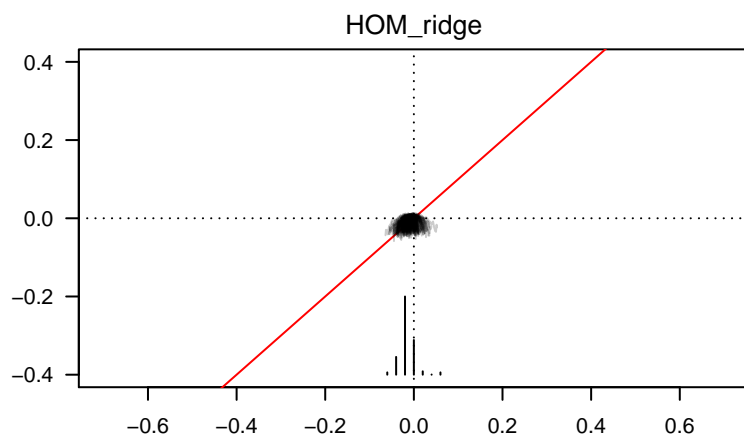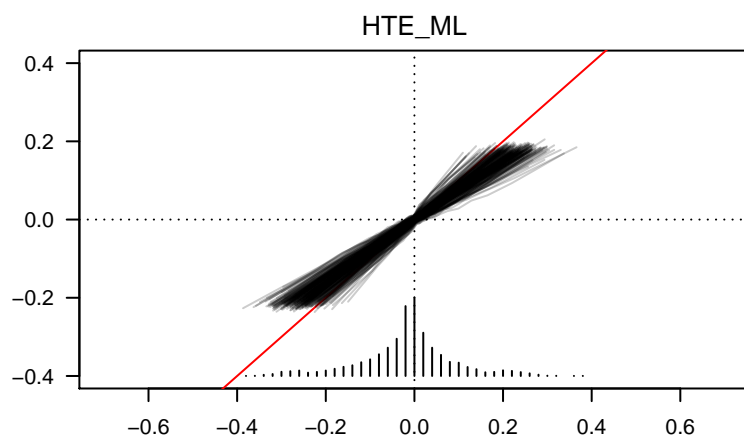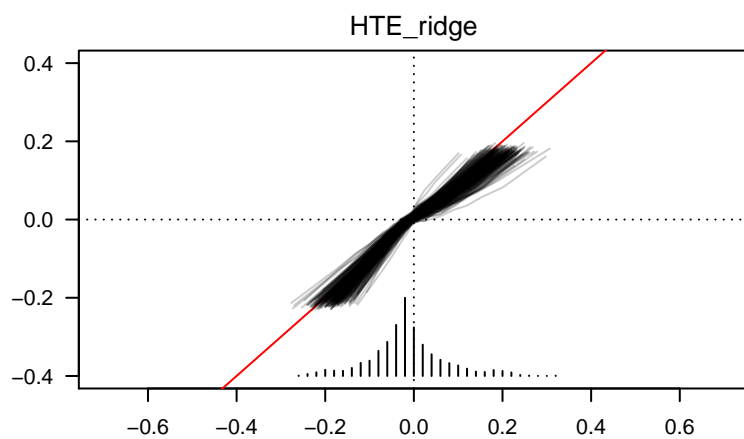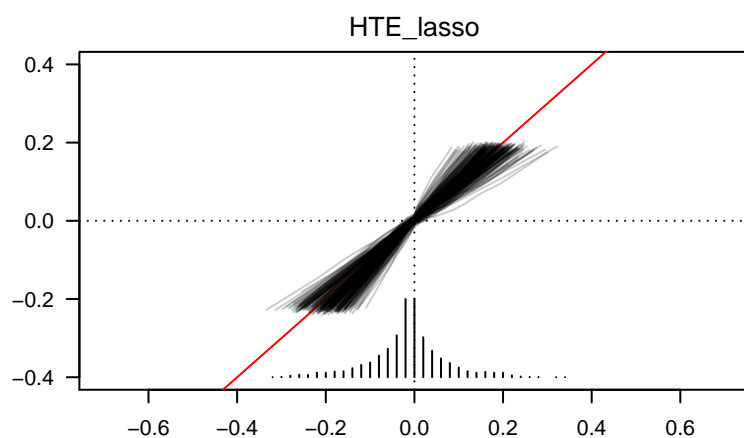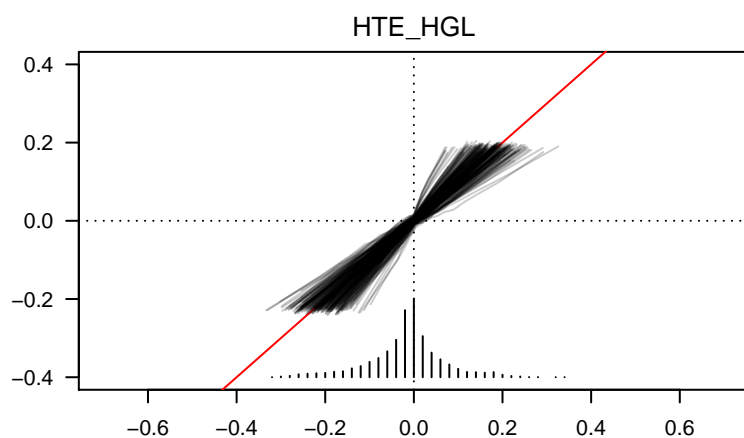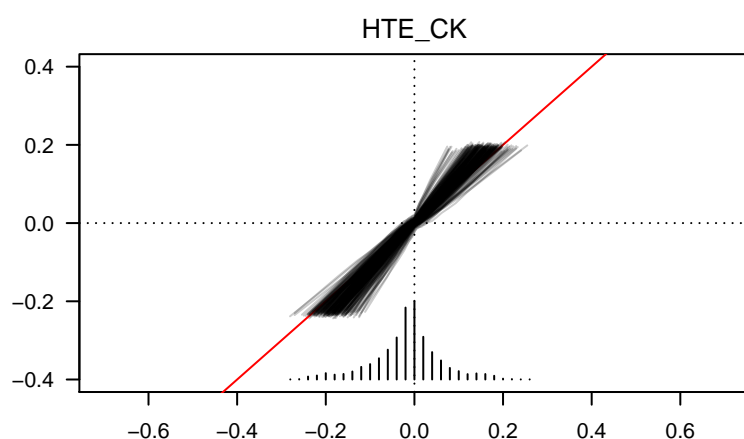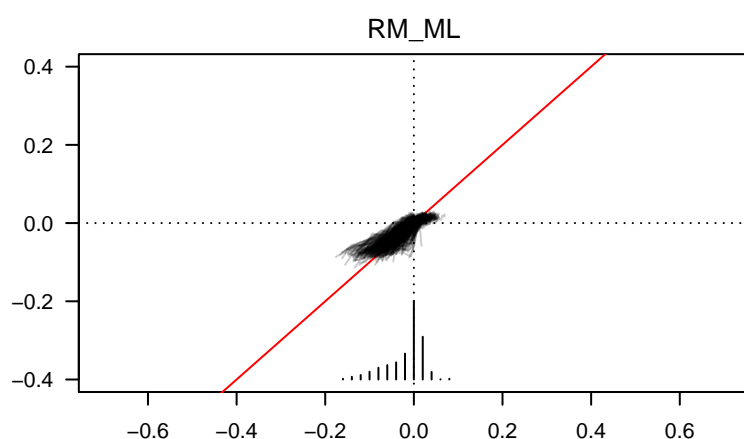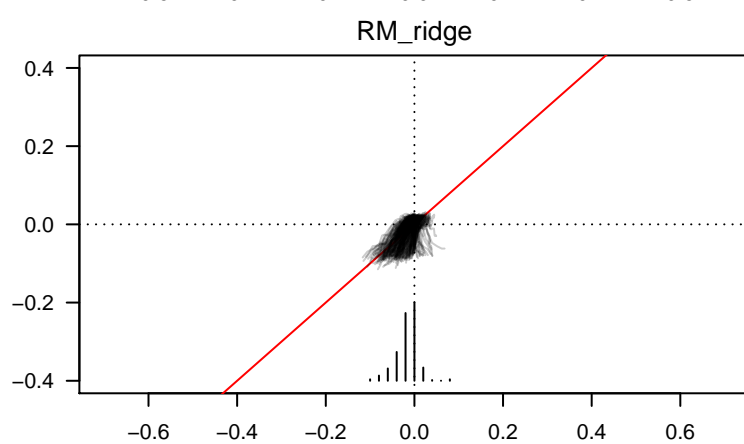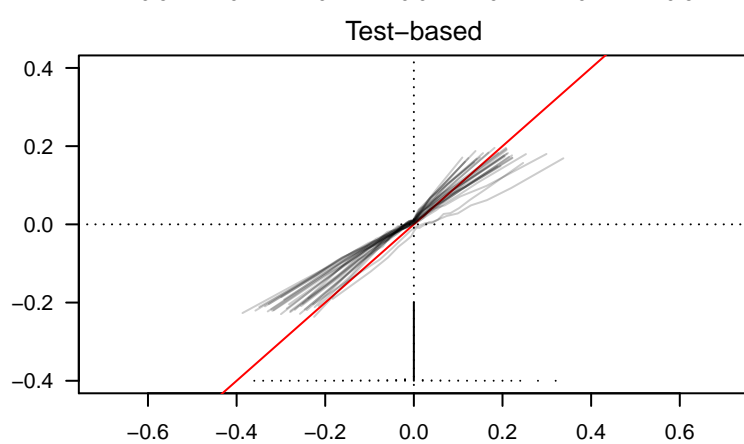

Supplement: Supplementary file 1 [file CalibrationFigures.pdf]
